# Supplementary material for: Luminosity Functions and Point Source Properties from Multiple Chandra Observations of M81
Source: arXiv:1104.2906 ancillary file (2011-04-14)
Supplement: Supplementary file 1 [file additional_tables.pdf]

TABLE 5
Merged Extraction Data of Sources in the Master and Borderline Source Lists

| Src Num | RA (degrees) | Dec (degrees) | Avg OAA (arcmin) | Tot Src Counts | Tot Bkg Counts | Soft Net Counts | Medium Net Counts | Hard Net Counts | PSF % | Var Stat 5935-5949 | Var Obs 5935-5949 | Var Stat merged-735 |
|---|---|---|---|---|---|---|---|---|---|---|---|---|
| 1 | 149.076036 | 68.822964 | 14.527 | 936 | 744.5 | $67.6^{+19.3}_{-18.3}$ | $93.4^{+15.1}_{-14.1}$ | $31.6^{+26.8}_{-25.8}$ | 90.0 | 1.78 | 5940.5945 | 1.44 |
| 2 | 149.113274 | 68.868505 | 12.209 | 807 | 591.2 | $51.3^{+18.0}_{-16.9}$ | $99.5^{+14.6}_{-13.5}$ | $65.0^{+25.0}_{-23.9}$ | 90.1 | 2.36 | 5937.5946 | 2.09 |
| 3 | 149.172497 | 68.888582 | 11.692 | 519 | 359.7 | $24.8^{+15.0}_{-14.0}$ | $82.1^{+12.8}_{-11.7}$ | $53.4^{+19.9}_{-18.9}$ | 90.0 | 3.18 | 5940.5945 | 2.49 |
| 4 | 149.162574 | 68.904939 | 10.738 | 150 | 105.9 | $5.1^{+7.9}_{-6.8}$ | $13.7^{+6.5}_{-5.5}$ | $25.3^{+11.6}_{-10.5}$ | 90.3 | 2.24 | 5942.5947 | 2.05 |
| 5 | 149.256021 | 68.916976 | 11.372 | 655 | 151.4 | $145.0^{+21.9}_{-20.9}$ | $250.3^{+17.7}_{-16.6}$ | $108.2^{+16.8}_{-15.7}$ | 90.3 | 4.55 | 5945.5948 | 3.59 |
| 6 | 148.776150 | 68.741468 | 19.003 | 207 | 129.0 | $17.7^{+10.2}_{-9.1}$ | $33.1^{+8.4}_{-7.3}$ | $28.2^{+12.7}_{-11.6}$ | 90.8 | 3.90 | 5937.5938 | 3.43 |
| 7 | 149.148898 | 68.762466 | 18.458 | 1481 | 1357.4 | $17.8^{+21.4}_{-20.4}$ | $70.5^{+17.6}_{-16.5}$ | $35.3^{+35.1}_{-34.1}$ | 90.1 | 2.99 | 5938.5948 | 2.66 |
| 8 | 149.378579 | 68.818487 | 17.638 | 981 | 758.1 | $62.7^{+19.8}_{-18.8}$ | $108.8^{+16.1}_{-15.1}$ | $51.4^{+27.3}_{-26.3}$ | 90.2 | 3.35 | 5947.5948 | 2.95 |
| 9 | 149.057171 | 68.956754 | 6.933 | 185 | 9.9 | $92.7^{+13.9}_{-12.8}$ | $69.3^{+9.5}_{-8.4}$ | $13.1^{+5.6}_{-4.4}$ | 69.5 | 1.95 | 5944.5948 | 1.44 |
| 10 | 148.799329 | 68.963358 | 5.865 | 46 | 8.8 | $6.0^{+5.9}_{-4.8}$ | $14.4^{+5.1}_{-4.0}$ | $16.8^{+5.9}_{-4.8}$ | 90.2 | 1.14 | 5936.5941 | 0.99 |
| 11 | 148.906715 | 68.975871 | 4.817 | 49 | 6.6 | $2.2^{+6.5}_{-5.4}$ | $24.8^{+6.2}_{-5.1}$ | $15.4^{+5.6}_{-4.4}$ | 89.9 | 1.33 | 5943.5946 | 1.11 |
| 12 | 148.955785 | 68.976906 | 4.941 | 551 | 7.3 | $148.9^{+21.7}_{-20.6}$ | $274.7^{+17.6}_{-16.6}$ | $121.2^{+12.3}_{-11.2}$ | 89.6 | 4.52 | 5936.5941 | 3.69 |
| 13 | 149.011250 | 68.979161 | 5.281 | 83 | 9.2 | $-0.4^{+6.6}_{-5.5}$ | $28.3^{+6.5}_{-5.4}$ | $45.9^{+8.3}_{-7.2}$ | 89.9 | 1.87 | 5939.5949 | 1.64 |
| 14 | 148.848781 | 68.980442 | 4.620 | 95 | 6.4 | $0.2^{+7.1}_{-6.1}$ | $34.9^{+7.1}_{-6.0}$ | $53.5^{+8.7}_{-7.6}$ | 90.0 | 1.93 | 5941.5946 | 1.71 |
| 15 | 148.773889 | 68.981398 | 5.093 | 29 | 5.9 | $16.2^{+6.1}_{-5.0}$ | $7.0^{+4.0}_{-2.8}$ | $-0.1^{+3.2}_{-1.9}$ | 90.4 | 1.42 | 5940.5941 | 1.29 |
| 16 | 149.008019 | 68.983260 | 5.030 | 99 | 7.9 | $24.8^{+9.5}_{-8.5}$ | $44.6^{+7.8}_{-6.8}$ | $21.7^{+6.3}_{-5.2}$ | 89.8 | 1.19 | 5935.5939 | 1.00 |
| 17 | 148.932216 | 68.984803 | 4.359 | 273 | 5.0 | $52.2^{+15.2}_{-14.1}$ | $146.1^{+13.2}_{-12.1}$ | $69.7^{+9.6}_{-8.5}$ | 90.0 | 3.42 | 5944.5946 | 2.38 |
| 18 | 148.971415 | 68.990641 | 4.281 | 798 | 5.1 | $103.2^{+23.3}_{-22.3}$ | $393.1^{+20.9}_{-19.8}$ | $296.6^{+18.3}_{-17.3}$ | 90.0 | 3.67 | 5940.5947 | 3.25 |
| 19 | 149.011061 | 68.993240 | 4.561 | 461 | 6.3 | $35.1^{+18.1}_{-17.0}$ | $253.9^{+17.0}_{-16.0}$ | $165.7^{+14.1}_{-13.0}$ | 90.3 | 2.28 | 5940.5948 | 1.70 |
| 20 | 149.151897 | 69.007926 | 6.190 | 209 | 4.8 | $47.4^{+13.7}_{-12.7}$ | $112.1^{+11.7}_{-10.6}$ | $45.7^{+8.1}_{-7.0}$ | 90.2 | 3.88 | 5945.5949 | 2.83 |
| 21 | 148.887313 | 69.009350 | 2.797 | 17705 | 2.6 | $2809.6^{+110.5}_{-109.5}$ | $9182.3^{+96.8}_{-95.8}$ | $5714.5^{+76.6}_{-75.6}$ | 89.6 | 4.93 | 5946.5947 | 3.75 |
| 22 | 148.978888 | 69.015550 | 3.071 | 513 | 2.4 | $98.6^{+20.5}_{-19.5}$ | $280.5^{+17.8}_{-16.8}$ | $131.4^{+12.6}_{-11.5}$ | 90.1 | 3.26 | 5935.5946 | 2.72 |
| 23 | 149.037425 | 69.018588 | 3.855 | 337 | 4.0 | $329.4^{+19.4}_{-18.3}$ | $6.3^{+3.8}_{-2.6}$ | $-0.6^{+2.7}_{-1.3}$ | 90.1 | 2.56 | 5937.5943 | 1.74 |
| 24 | 149.013452 | 69.018800 | 3.443 | 38 | 3.0 | $9.5^{+6.1}_{-5.0}$ | $14.4^{+5.0}_{-3.8}$ | $11.0^{+4.7}_{-3.6}$ | 89.8 | 1.23 | 5938.5946 | 1.17 |
| 25 | 148.890742 | 69.023304 | 1.966 | 16 | 1.1 | $3.8^{+4.1}_{-2.9}$ | $4.7^{+3.4}_{-2.2}$ | $6.4^{+3.8}_{-2.6}$ | 90.1 | 0.93 | 5935.5936 | 0.87 |
| 26 | 148.953212 | 69.027876 | 2.144 | 12 | 1.3 | $-0.2^{+3.8}_{-2.6}$ | $6.7^{+3.8}_{-2.6}$ | $4.2^{+3.4}_{-2.2}$ | 89.6 | 0.91 | 5935.5947 | 0.89 |
| 27 | 149.033648 | 69.028530 | 3.474 | 13 | 3.8 | $0.3^{+3.8}_{-2.6}$ | $5.3^{+3.6}_{-2.4}$ | $3.6^{+3.6}_{-2.4}$ | 89.8 | 0.92 | 5936.5939 | 0.87 |
| 28 | 149.082560 | 69.033797 | 4.274 | 60 | 3.6 | $3.3^{+6.0}_{-4.9}$ | $19.3^{+5.6}_{-4.4}$ | $33.7^{+7.1}_{-6.0}$ | 90.0 | 1.64 | 5945.5949 | 1.44 |
| 29 | 149.070613 | 68.972373 | 6.308 | 222 | 13.1 | $30.1^{+12.9}_{-11.8}$ | $105.6^{+11.4}_{-10.4}$ | $73.2^{+10.1}_{-9.0}$ | 90.0 | 1.71 | 5939.5944 | 1.93 |
| 30 | 149.019710 | 68.978065 | 5.433 | 68 | 9.2 | $5.7^{+7.2}_{-6.1}$ | $29.3^{+6.6}_{-5.5}$ | $23.8^{+6.5}_{-5.4}$ | 89.8 | 0.96 | 5940.5946 | 0.74 |
| 31 | 148.838419 | 68.982119 | 4.571 | 39 | 6.3 | $9.2^{+6.4}_{-5.3}$ | $16.9^{+5.3}_{-4.2}$ | $6.7^{+4.4}_{-3.3}$ | 89.8 | 1.44 | 5941.5949 | 1.37 |
| 32 | 148.825959 | 68.991776 | 4.094 | 27 | 4.7 | $2.4^{+4.8}_{-3.7}$ | $10.2^{+4.4}_{-3.3}$ | $9.8^{+4.7}_{-3.6}$ | 89.9 | 1.22 | 5936.5945 | 1.14 |
| 33 | 149.025047 | 68.994865 | 4.660 | 81 | 6.4 | $-0.9^{+2.3}_{-0.8}$ | $-0.2^{+2.3}_{-0.8}$ | $75.7^{+10.0}_{-8.9}$ | 89.8 | 1.48 | 5937.5940 | 1.39 |
| 34 | 149.100032 | 69.002707 | 5.461 | 36 | 6.4 | $2.2^{+5.7}_{-4.5}$ | $16.8^{+5.3}_{-4.2}$ | $10.6^{+5.0}_{-3.8}$ | 89.8 | 0.84 | 5943.5947 | 0.86 |
| 35 | 149.117048 | 69.017175 | 5.293 | 71 | 4.1 | $6.4^{+7.9}_{-6.8}$ | $39.2^{+7.4}_{-6.3}$ | $21.2^{+6.0}_{-4.9}$ | 89.5 | 1.09 | 5943.5944 | 1.06 |
| 36 | 148.919472 | 69.018108 | 2.352 | 10 | 1.8 | $1.7^{+3.8}_{-2.6}$ | $4.6^{+3.4}_{-2.2}$ | $1.9^{+2.9}_{-1.6}$ | 90.0 | 0.90 | 5935.5947 | 0.88 |
| 37 | 149.213828 | 68.935057 | 9.965 | 197 | 30.3 | $15.3^{+11.9}_{-10.8}$ | $93.1^{+11.0}_{-9.9}$ | $58.3^{+10.0}_{-9.0}$ | 90.1 | 4.13 | 5944.5947 | 3.46 |
| 38 | 148.761134 | 68.939388 | 7.481 | 49 | 5.6 | $26.4^{+7.8}_{-6.7}$ | $17.1^{+5.3}_{-4.2}$ | $-0.2^{+3.2}_{-1.9}$ | 59.5 | 1.91 | 5937.5940 | 1.49 |
| 39 | 148.754210 | 68.939329 | 7.537 | 73 | 5.3 | $49.5^{+9.4}_{-8.3}$ | $18.2^{+5.4}_{-4.3}$ | $0.0^{+3.2}_{-1.9}$ | 59.7 | 1.99 | 5938.5940 | 1.77 |
| 40 | 148.903499 | 68.948983 | 6.416 | 106 | 18.5 | $12.5^{+9.4}_{-8.3}$ | $52.0^{+8.5}_{-7.4}$ | $23.0^{+7.1}_{-6.0}$ | 90.0 | 1.12 | 5942.5944 | 1.16 |
| 41 | 149.061927 | 68.959075 | 6.866 | 110 | 9.4 | $14.8^{+8.9}_{-7.9}$ | $44.4^{+7.8}_{-6.8}$ | $41.5^{+8.0}_{-6.9}$ | 69.4 | 1.87 | 5935.5948 | 1.67 |
| 42 | 148.960863 | 68.975506 | 5.053 | 57 | 7.9 | $1.9^{+6.6}_{-5.5}$ | $26.6^{+6.4}_{-5.3}$ | $20.7^{+6.2}_{-5.1}$ | 89.8 | 1.47 | 5940.5944 | 1.24 |

TABLE 5 — *Continued*

| Src Num | RA (degrees) | Dec (degrees) | Avg OAA (arcmin) | Tot Src Counts | Tot Bkg Counts | Soft Net Counts | Medium Net Counts | Hard Net Counts | PSF % | Var Stat 5935-5949 | Var Obs 5935-5949 | Var Stat merged-735 |
|---|---|---|---|---|---|---|---|---|---|---|---|---|
| 43 | 148.950816 | 68.987692 | 4.291 | 20 | 4.9 | $10.2^{+5.3}_{-4.2}$ | $6.1^{+3.8}_{-2.6}$ | $-1.2^{+2.7}_{-1.3}$ | 90.0 | 1.21 | 5935.5948 | 1.15 |
| 44 | 149.068123 | 69.022042 | 4.290 | 24 | 4.6 | $-0.8^{+2.7}_{-1.3}$ | $1.1^{+2.7}_{-1.3}$ | $19.1^{+5.8}_{-4.7}$ | 89.8 | 1.23 | 5936.5940 | 1.19 |
| 45 | 149.128064 | 69.039230 | 5.045 | 16 | 1.9 | $0.8^{+4.0}_{-2.8}$ | $6.6^{+3.8}_{-2.6}$ | $6.7^{+4.0}_{-2.8}$ | 89.7 | 0.66 | 5945.5947 | 0.50 |
| 46 | 148.787915 | 68.893381 | 9.968 | 95 | 42.2 | $4.4^{+8.4}_{-7.4}$ | $38.5^{+7.8}_{-6.7}$ | $9.8^{+7.6}_{-6.5}$ | 90.5 | 1.30 | 5939.5941 | 1.07 |
| 47 | 148.897110 | 68.919941 | 8.155 | 107 | 36.9 | $19.5^{+9.5}_{-8.4}$ | $42.2^{+8.0}_{-6.9}$ | $8.4^{+7.1}_{-6.0}$ | 90.3 | 1.58 | 5941.5945 | 1.49 |
| 48 | 149.257594 | 68.947923 | 10.100 | 168 | 21.9 | $17.7^{+11.0}_{-9.9}$ | $73.9^{+9.9}_{-8.8}$ | $54.4^{+9.5}_{-8.4}$ | 90.2 | 1.70 | 5946.5949 | 1.30 |
| 49 | 149.129387 | 68.977177 | 6.911 | 35 | 11.3 | $0.6^{+4.8}_{-3.7}$ | $10.0^{+4.6}_{-3.4}$ | $13.0^{+5.7}_{-4.6}$ | 90.0 | 1.33 | 5939.5948 | 1.29 |
| 50 | 148.949479 | 68.991232 | 4.080 | 17 | 4.2 | $13.3^{+5.1}_{-4.0}$ | $1.2^{+2.7}_{-1.3}$ | $-1.7^{+2.3}_{-0.8}$ | 90.2 | 0.89 | 5938.5939 | 0.82 |
| 51 | 149.093012 | 69.038619 | 4.376 | 23 | 2.8 | $1.5^{+5.3}_{-4.2}$ | $15.5^{+5.1}_{-4.0}$ | $3.2^{+3.4}_{-2.2}$ | 89.7 | 1.36 | 5940.5944 | 1.27 |
| 52 | 148.951534 | 68.899759 | 9.458 | 66 | 23.9 | $4.6^{+6.7}_{-5.6}$ | $20.8^{+6.1}_{-5.0}$ | $16.7^{+6.9}_{-5.8}$ | 60.2 | 1.25 | 5946.5948 | 1.03 |
| 53 | 148.968276 | 68.940319 | 7.133 | 44 | 23.0 | $0.5^{+4.9}_{-3.7}$ | $6.9^{+4.4}_{-3.3}$ | $13.6^{+6.6}_{-5.5}$ | 89.6 | 1.26 | 5937.5947 | 1.26 |
| 54 | 149.069525 | 68.947443 | 7.541 | 68 | 24.4 | $0.8^{+6.5}_{-5.4}$ | $21.2^{+6.1}_{-5.0}$ | $21.6^{+7.3}_{-6.2}$ | 90.2 | 1.50 | 5936.5944 | 1.42 |
| 55 | 149.136025 | 68.954438 | 8.006 | 58 | 20.7 | $0.6^{+5.7}_{-4.6}$ | $14.7^{+5.3}_{-4.2}$ | $22.0^{+7.2}_{-6.1}$ | 90.1 | 1.64 | 5944.5948 | 1.53 |
| 56 | 149.211953 | 68.976997 | 8.252 | 28 | 11.9 | $1.8^{+4.7}_{-3.6}$ | $7.8^{+4.3}_{-3.1}$ | $6.5^{+5.0}_{-3.9}$ | 89.9 | 0.38 | 5947.5948 | 0.25 |
| 57 | 149.174769 | 68.982774 | 7.417 | 32 | 9.7 | $0.7^{+5.0}_{-3.8}$ | $11.4^{+4.7}_{-3.6}$ | $10.3^{+5.2}_{-4.1}$ | 90.0 | 1.58 | 5944.5947 | 1.44 |
| 58 | 149.139856 | 69.010495 | 5.899 | 22 | 4.7 | $1.4^{+4.7}_{-3.6}$ | $10.1^{+4.4}_{-3.3}$ | $5.7^{+4.1}_{-2.9}$ | 89.6 | 1.07 | 5943.5946 | 0.95 |
| 59 | 148.756021 | 68.891831 | 10.219 | 73 | 30.5 | $4.6^{+6.8}_{-5.7}$ | $19.5^{+6.0}_{-4.9}$ | $18.3^{+7.6}_{-6.5}$ | 89.9 | 1.18 | 5937.5938 | 0.87 |
| 60 | 148.942950 | 68.895185 | 9.707 | 56 | 25.8 | $7.3^{+6.5}_{-5.4}$ | $14.8^{+5.5}_{-4.3}$ | $8.1^{+6.3}_{-5.2}$ | 58.5 | 1.07 | 5937.5943 | 1.04 |
| 61 | 149.051454 | 68.903776 | 9.755 | 127 | 70.6 | $5.0^{+8.0}_{-7.0}$ | $23.4^{+7.1}_{-6.0}$ | $28.1^{+10.0}_{-9.0}$ | 89.5 | 1.59 | 5935.5938 | 1.55 |
| 62 | 148.853193 | 69.020468 | 2.293 | 3385 | 1.6 | $1510.8^{+56.9}_{-55.9}$ | $1610.6^{+41.1}_{-40.1}$ | $264.0^{+17.3}_{-16.3}$ | 89.4 | 2.46 | 5946.5948 | 2.39 |
| 63 | 148.801598 | 69.022653 | 2.790 | 53 | 2.6 | $11.7^{+6.5}_{-5.4}$ | $16.5^{+5.2}_{-4.1}$ | $22.2^{+6.0}_{-4.9}$ | 89.8 | 1.56 | 5940.5947 | 1.29 |
| 64 | 148.879558 | 69.028900 | 1.646 | 10 | 2.1 | $0.6^{+2.7}_{-1.3}$ | $0.5^{+2.3}_{-0.8}$ | $6.8^{+4.0}_{-2.8}$ | 90.0 | 0.73 | 5935.5936 | 0.69 |
| 65 | 148.751372 | 69.030273 | 3.381 | 69 | 4.6 | $2.4^{+5.8}_{-4.7}$ | $18.0^{+5.4}_{-4.3}$ | $44.0^{+7.9}_{-6.8}$ | 89.8 | 1.78 | 5940.5942 | 1.67 |
| 66 | 148.971794 | 69.035277 | 2.163 | 71 | 1.7 | $7.7^{+8.0}_{-6.9}$ | $39.6^{+7.4}_{-6.3}$ | $22.0^{+5.9}_{-4.8}$ | 89.4 | 1.75 | 5939.5944 | 1.49 |
| 67 | 148.905243 | 69.035413 | 1.272 | 33 | 2.4 | $14.4^{+6.3}_{-5.2}$ | $11.5^{+4.6}_{-3.4}$ | $4.7^{+3.6}_{-2.4}$ | 90.5 | 1.48 | 5938.5943 | 1.28 |
| 68 | 149.012509 | 69.038167 | 2.835 | 50 | 2.9 | $5.4^{+6.6}_{-5.5}$ | $24.4^{+6.1}_{-5.0}$ | $17.2^{+5.4}_{-4.3}$ | 89.9 | 1.52 | 5942.5948 | 1.35 |
| 69 | 148.939187 | 69.038215 | 1.484 | 15 | 2.3 | $-0.5^{+3.2}_{-1.9}$ | $3.5^{+3.2}_{-1.9}$ | $9.7^{+4.4}_{-3.3}$ | 90.0 | 0.87 | 5939.5948 | 0.79 |
| 70 | 148.841656 | 69.041321 | 1.376 | 23 | 2.2 | $3.5^{+5.1}_{-4.0}$ | $11.5^{+4.6}_{-3.4}$ | $5.8^{+3.8}_{-2.6}$ | 90.4 | 1.24 | 5940.5944 | 1.13 |
| 71 | 148.813370 | 69.041841 | 1.868 | 33 | 2.0 | $0.7^{+4.4}_{-3.3}$ | $9.5^{+4.3}_{-3.1}$ | $20.8^{+5.8}_{-4.7}$ | 89.6 | 1.29 | 5936.5942 | 1.29 |
| 72 | 148.885832 | 69.042135 | 0.842 | 139 | 2.5 | $16.2^{+10.3}_{-9.3}$ | $68.5^{+9.4}_{-8.3}$ | $51.9^{+8.3}_{-7.3}$ | 90.4 | 1.52 | 5939.5948 | 1.60 |
| 73 | 148.978970 | 69.044224 | 2.018 | 124 | 2.6 | $38.5^{+10.7}_{-9.6}$ | $53.4^{+8.4}_{-7.3}$ | $29.5^{+6.6}_{-5.5}$ | 89.7 | 1.94 | 5942.5947 | 1.67 |
| 74 | 148.739953 | 69.044800 | 3.309 | 436 | 5.1 | $99.3^{+18.8}_{-17.8}$ | $216.0^{+15.8}_{-14.7}$ | $115.6^{+11.9}_{-10.9}$ | 89.9 | 3.53 | 5938.5948 | 2.94 |
| 75 | 148.868438 | 69.045753 | 0.784 | 73 | 2.6 | $69.2^{+9.5}_{-8.4}$ | $0.4^{+2.3}_{-0.8}$ | $0.9^{+2.7}_{-1.3}$ | 90.4 | 1.76 | 5936.5945 | 1.76 |
| 76 | 148.901025 | 69.045855 | 0.650 | 22 | 2.9 | $12.9^{+5.7}_{-4.5}$ | $6.3^{+3.8}_{-2.6}$ | $0.8^{+2.7}_{-1.3}$ | 90.3 | 1.05 | 5940.5949 | 0.94 |
| 77 | 148.876007 | 69.046364 | 0.665 | 45 | 2.8 | $11.1^{+6.7}_{-5.6}$ | $19.3^{+5.6}_{-4.4}$ | $11.8^{+4.7}_{-3.6}$ | 90.3 | 1.43 | 5936.5945 | 1.15 |
| 78 | 148.863572 | 69.046689 | 0.812 | 367 | 2.5 | $76.2^{+17.1}_{-16.1}$ | $180.4^{+14.5}_{-13.4}$ | $107.9^{+11.5}_{-10.4}$ | 90.4 | 2.14 | 5946.5947 | 2.11 |
| 79 | 149.059826 | 69.046840 | 3.677 | 132 | 4.8 | $24.1^{+10.6}_{-9.5}$ | $65.1^{+9.2}_{-8.1}$ | $38.0^{+7.5}_{-6.4}$ | 89.9 | 2.22 | 5939.5942 | 2.02 |
| 80 | 148.894040 | 69.047278 | 0.535 | 297 | 3.1 | $60.8^{+15.5}_{-14.5}$ | $147.2^{+13.2}_{-12.2}$ | $86.8^{+10.4}_{-9.4}$ | 90.3 | 1.87 | 5947.5948 | 1.34 |
| 81 | 148.938964 | 69.048318 | 1.126 | 19 | 2.4 | $15.3^{+5.4}_{-4.3}$ | $2.4^{+2.9}_{-1.6}$ | $-1.2^{+1.9}_{-nan}$ | 90.5 | 0.89 | 5935.5939 | 0.75 |
| 82 | 148.919792 | 69.049553 | 0.729 | 21 | 3.1 | $3.9^{+4.8}_{-3.7}$ | $8.2^{+4.1}_{-2.9}$ | $5.7^{+3.8}_{-2.6}$ | 90.5 | 1.21 | 5935.5939 | 1.14 |
| 83 | 148.957492 | 69.050061 | 1.467 | 16 | 2.5 | $0.5^{+4.4}_{-3.3}$ | $9.5^{+4.3}_{-3.1}$ | $3.6^{+3.4}_{-2.2}$ | 90.0 | 0.88 | 5937.5939 | 0.78 |
| 84 | 148.941116 | 69.050128 | 1.130 | 308 | 2.6 | $73.3^{+16.2}_{-15.2}$ | $156.4^{+13.6}_{-12.5}$ | $75.7^{+9.8}_{-8.8}$ | 90.6 | 2.06 | 5936.5949 | 1.57 |
| 85 | 148.924628 | 69.050560 | 0.791 | 16 | 3.1 | $1.9^{+4.3}_{-3.1}$ | $6.3^{+3.8}_{-2.6}$ | $4.7^{+3.6}_{-2.4}$ | 90.5 | 0.85 | 5935.5939 | 0.72 |

TABLE 5 — *Continued*

| Src Num | RA (degrees) | Dec (degrees) | Avg OAA (arcmin) | Tot Src Counts | Tot Bkg Counts | Soft Net Counts | Medium Net Counts | Hard Net Counts | PSF % | Var Stat 5935-5949 | Var Obs 5935-5949 | Var Stat merged-735 |
|---|---|---|---|---|---|---|---|---|---|---|---|---|
| 86 | 148.968691 | 69.051699 | 1.685 | 1968 | 2.4 | $449.5^{+37.5}_{-36.5}$ | $883.4^{+30.7}_{-29.7}$ | $637.6^{+26.3}_{-25.3}$ | 89.7 | 6.51 | 5937.5944 | 4.80 |
| 87 | 148.983487 | 69.053378 | 1.988 | 61 | 2.4 | $48.5^{+8.8}_{-7.7}$ | $10.5^{+4.4}_{-3.3}$ | $0.6^{+2.7}_{-1.3}$ | 89.6 | 0.70 | 5936.5942 | 0.49 |
| 88 | 148.837600 | 69.053686 | 1.152 | 20 | 2.3 | $7.5^{+5.0}_{-3.8}$ | $6.4^{+3.8}_{-2.6}$ | $3.8^{+3.4}_{-2.2}$ | 90.6 | 1.07 | 5935.5940 | 0.99 |
| 89 | 148.918163 | 69.054102 | 0.593 | 38 | 3.7 | $10.6^{+6.3}_{-5.2}$ | $14.1^{+5.0}_{-3.8}$ | $9.7^{+4.4}_{-3.3}$ | 90.4 | 1.58 | 5941.5948 | 1.40 |
| 90 | 148.896851 | 69.054471 | 0.178 | 827 | 4.4 | $198.3^{+25.5}_{-24.5}$ | $399.8^{+21.0}_{-20.0}$ | $225.5^{+16.1}_{-15.1}$ | 90.2 | 3.83 | 5935.5942 | 2.89 |
| 91 | 148.875598 | 69.055122 | 0.335 | 149 | 3.8 | $43.6^{+11.6}_{-10.6}$ | $66.0^{+9.2}_{-8.2}$ | $35.6^{+7.1}_{-6.1}$ | 90.3 | 1.87 | 5937.5949 | 1.40 |
| 92 | 148.927251 | 69.055601 | 0.777 | 266 | 3.4 | $80.7^{+15.0}_{-14.0}$ | $113.2^{+11.7}_{-10.7}$ | $68.7^{+9.4}_{-8.3}$ | 90.6 | 4.54 | 5942.5948 | 4.03 |
| 93 | 148.871493 | 69.055830 | 0.419 | 93 | 3.7 | $30.7^{+9.4}_{-8.3}$ | $36.0^{+7.1}_{-6.1}$ | $22.6^{+6.0}_{-4.9}$ | 90.4 | 1.17 | 5941.5942 | 0.91 |
| 94 | 149.032255 | 69.057045 | 3.035 | 106 | 4.1 | $15.3^{+9.1}_{-8.0}$ | $48.2^{+8.1}_{-7.0}$ | $38.4^{+7.5}_{-6.4}$ | 89.8 | 1.77 | 5937.5948 | 1.38 |
| 95 | 148.907452 | 69.057781 | 0.370 | 28 | 4.9 | $11.0^{+5.9}_{-4.8}$ | $8.7^{+4.3}_{-3.1}$ | $3.4^{+3.4}_{-2.2}$ | 90.3 | 1.31 | 5938.5942 | 1.18 |
| 96 | 148.925608 | 69.060142 | 0.782 | 1906 | 3.7 | $1839.6^{+45.1}_{-44.1}$ | $102.1^{+11.2}_{-10.1}$ | $1.6^{+2.9}_{-1.6}$ | 90.6 | 15.03 | 5943.5947 | 12.76 |
| 97 | 148.893780 | 69.060837 | 0.322 | 76 | 7.2 | $19.2^{+7.8}_{-6.8}$ | $21.7^{+6.0}_{-4.9}$ | $28.0^{+6.5}_{-5.4}$ | 90.3 | 1.00 | 5937.5942 | 0.81 |
| 98 | 149.061114 | 69.060846 | 3.663 | 95 | 5.6 | $7.2^{+8.3}_{-7.3}$ | $43.7^{+7.8}_{-6.7}$ | $38.5^{+7.5}_{-6.5}$ | 89.6 | 1.81 | 5943.5945 | 1.45 |
| 99 | 148.878388 | 69.061768 | 0.456 | 31 | 2.7 | $4.9^{+6.2}_{-5.1}$ | $19.1^{+5.6}_{-4.4}$ | $4.3^{+3.4}_{-2.2}$ | 69.6 | 1.06 | 5936.5949 | 1.03 |
| 100 | 148.895425 | 69.061806 | 0.383 | 1715 | 8.2 | $306.7^{+34.1}_{-33.1}$ | $783.4^{+29.0}_{-28.0}$ | $617.8^{+25.9}_{-24.9}$ | 90.4 | 5.90 | 5938.5946 | 4.42 |
| 101 | 148.840646 | 69.062508 | 1.154 | 48 | 2.6 | $7.3^{+6.4}_{-5.3}$ | $19.3^{+5.6}_{-4.4}$ | $18.7^{+5.6}_{-4.4}$ | 90.1 | 1.44 | 5942.5944 | 1.26 |
| 102 | 148.975709 | 69.062955 | 1.862 | 43 | 2.4 | $16.5^{+7.1}_{-6.1}$ | $19.5^{+5.6}_{-4.4}$ | $4.7^{+3.6}_{-2.4}$ | 89.7 | 1.59 | 5937.5938 | 1.32 |
| 103 | 148.892885 | 69.063294 | 0.459 | 102 | 12.8 | $33.8^{+10.2}_{-9.1}$ | $40.7^{+7.8}_{-6.7}$ | $14.8^{+5.3}_{-4.2}$ | 90.5 | 1.07 | 5947.5949 | 0.81 |
| 104 | 148.916509 | 69.063564 | 0.715 | 24 | 5.2 | $-1.3^{+4.4}_{-3.3}$ | $8.7^{+4.3}_{-3.1}$ | $11.3^{+4.7}_{-3.6}$ | 90.6 | 1.33 | 5938.5946 | 1.25 |
| 105 | 148.892901 | 69.064138 | 0.509 | 458 | 7.2 | $130.0^{+19.5}_{-18.5}$ | $205.6^{+15.4}_{-14.4}$ | $115.3^{+11.9}_{-10.8}$ | 79.8 | 2.16 | 5938.5942 | 1.98 |
| 106 | 148.894573 | 69.064390 | 0.527 | 379 | 6.5 | $52.2^{+14.7}_{-13.7}$ | $130.8^{+12.6}_{-11.5}$ | $189.4^{+14.8}_{-13.8}$ | 79.8 | 4.63 | 5936.5938 | 4.15 |
| 107 | 148.832922 | 69.064366 | 1.348 | 21 | 2.4 | $0.4^{+4.0}_{-2.8}$ | $6.4^{+3.8}_{-2.6}$ | $11.7^{+4.7}_{-3.6}$ | 90.0 | 1.05 | 5938.5943 | 0.86 |
| 108 | 148.897433 | 69.064623 | 0.551 | 651 | 10.5 | $171.4^{+22.8}_{-21.8}$ | $295.7^{+18.3}_{-17.3}$ | $173.3^{+14.3}_{-13.3}$ | 90.5 | 3.32 | 5938.5945 | 2.65 |
| 109 | 148.931535 | 69.065459 | 1.041 | 33 | 3.2 | $8.9^{+6.1}_{-5.0}$ | $14.3^{+5.0}_{-3.8}$ | $6.7^{+4.0}_{-2.8}$ | 90.4 | 1.21 | 5944.5947 | 1.05 |
| 110 | 148.983738 | 69.066219 | 2.081 | 23 | 2.6 | $7.5^{+5.6}_{-4.4}$ | $11.4^{+4.6}_{-3.4}$ | $1.5^{+2.9}_{-1.6}$ | 89.4 | 1.22 | 5935.5949 | 1.12 |
| 111 | 148.865846 | 69.066842 | 0.855 | 178 | 8.0 | $43.7^{+12.7}_{-11.6}$ | $86.6^{+10.5}_{-9.4}$ | $39.8^{+7.5}_{-6.5}$ | 90.8 | 1.45 | 5948.5949 | 1.05 |
| 112 | 148.860255 | 69.066856 | 0.936 | 57 | 5.1 | $11.1^{+7.5}_{-6.4}$ | $26.5^{+6.4}_{-5.3}$ | $14.4^{+5.1}_{-4.0}$ | 90.4 | 0.89 | 5936.5942 | 0.70 |
| 113 | 148.887951 | 69.067659 | 0.718 | 114 | 18.1 | $23.1^{+10.0}_{-8.9}$ | $43.0^{+8.1}_{-7.0}$ | $29.8^{+6.9}_{-5.8}$ | 90.6 | 1.45 | 5937.5943 | 1.26 |
| 114 | 148.776394 | 69.068220 | 2.567 | 116 | 3.1 | $36.5^{+10.6}_{-9.5}$ | $53.3^{+8.4}_{-7.3}$ | $23.0^{+6.1}_{-5.0}$ | 90.0 | 2.42 | 5936.5944 | 2.12 |
| 115 | 148.885381 | 69.068884 | 0.797 | 45 | 16.5 | $6.7^{+7.2}_{-6.1}$ | $17.6^{+5.9}_{-4.8}$ | $4.2^{+4.0}_{-2.8}$ | 90.7 | 1.60 | 5936.5942 | 1.52 |
| 116 | 148.790629 | 69.068813 | 2.289 | 187 | 2.6 | $30.6^{+12.9}_{-11.9}$ | $109.4^{+11.5}_{-10.5}$ | $44.4^{+7.8}_{-6.8}$ | 89.6 | 1.22 | 5938.5949 | 1.02 |
| 117 | 148.895316 | 69.068945 | 0.796 | 394 | 10.2 | $91.8^{+17.5}_{-16.4}$ | $170.9^{+14.2}_{-13.2}$ | $121.1^{+12.2}_{-11.1}$ | 90.7 | 1.59 | 5943.5945 | 1.33 |
| 118 | 148.801573 | 69.070039 | 2.098 | 17 | 2.5 | $5.5^{+4.4}_{-3.3}$ | $4.4^{+3.4}_{-2.2}$ | $5.5^{+3.8}_{-2.6}$ | 89.3 | 0.68 | 5935.5945 | 0.51 |
| 119 | 148.877083 | 69.071130 | 0.968 | 78 | 9.0 | $9.3^{+9.0}_{-8.0}$ | $48.2^{+8.2}_{-7.1}$ | $11.5^{+4.8}_{-3.7}$ | 90.8 | 1.75 | 5939.5947 | 1.50 |
| 120 | 149.000727 | 69.071874 | 2.537 | 34 | 2.0 | $25.7^{+6.6}_{-5.5}$ | $4.6^{+3.4}_{-2.2}$ | $1.8^{+2.9}_{-1.6}$ | 79.3 | 1.09 | 5941.5948 | 1.04 |
| 121 | 148.880380 | 69.072037 | 1.001 | 578 | 7.3 | $123.0^{+21.2}_{-20.1}$ | $277.9^{+17.8}_{-16.7}$ | $170.8^{+14.2}_{-13.1}$ | 90.7 | 4.00 | 5939.5942 | 3.16 |
| 122 | 148.729436 | 69.072125 | 3.597 | 28 | 5.6 | $7.3^{+5.4}_{-4.3}$ | $9.8^{+4.4}_{-3.3}$ | $5.3^{+4.1}_{-2.9}$ | 89.7 | 1.58 | 5940.5948 | 1.51 |
| 123 | 148.912252 | 69.073132 | 1.133 | 43 | 4.5 | $1.1^{+6.2}_{-5.1}$ | $22.0^{+5.9}_{-4.8}$ | $15.5^{+5.2}_{-4.1}$ | 89.7 | 1.23 | 5936.5943 | 1.03 |
| 124 | 148.886296 | 69.073144 | 1.046 | 24 | 6.1 | $0.5^{+5.0}_{-3.8}$ | $10.4^{+4.6}_{-3.4}$ | $7.0^{+4.1}_{-2.9}$ | 90.7 | 1.16 | 5940.5946 | 1.04 |
| 125 | 148.930324 | 69.073230 | 1.342 | 56 | 3.0 | $-0.0^{+2.9}_{-1.6}$ | $1.3^{+2.7}_{-1.3}$ | $51.7^{+8.3}_{-7.3}$ | 89.6 | 1.67 | 5936.5940 | 1.61 |
| 126 | 148.904123 | 69.075936 | 1.239 | 462 | 4.8 | $125.1^{+19.8}_{-18.8}$ | $224.9^{+16.1}_{-15.0}$ | $107.3^{+11.5}_{-10.4}$ | 89.6 | 4.74 | 5944.5948 | 4.49 |
| 127 | 148.973342 | 69.076338 | 2.150 | 153 | 2.6 | $36.5^{+11.7}_{-10.7}$ | $76.4^{+9.8}_{-8.8}$ | $37.5^{+7.3}_{-6.2}$ | 89.9 | 1.41 | 5937.5944 | 1.14 |
| 128 | 148.990198 | 69.076744 | 2.467 | 692 | 3.2 | $222.4^{+25.3}_{-24.3}$ | $365.3^{+20.2}_{-19.1}$ | $104.1^{+11.3}_{-10.3}$ | 89.5 | 5.77 | 5939.5949 | 4.37 |

TABLE 5 — *Continued*

| Src Num | RA (degrees) | Dec (degrees) | Avg OAA (arcmin) | Tot Src Counts | Tot Bkg Counts | Soft Net Counts | Medium Net Counts | Hard Net Counts | PSF % | Var Stat 5935-5949 | Var Obs 5935-5949 | Var Stat merged-735 |
|---|---|---|---|---|---|---|---|---|---|---|---|---|
| 129 | 148.750841 | 69.077046 | 3.260 | 41 | 4.6 | $3.4^{+5.9}_{-4.8}$ | $18.1^{+5.4}_{-4.3}$ | $15.0^{+5.3}_{-4.2}$ | 89.7 | 1.46 | 5938.5948 | 1.27 |
| 130 | 148.745141 | 69.077423 | 3.383 | 32 | 4.9 | $-0.7^{+5.3}_{-4.2}$ | $17.0^{+5.3}_{-4.2}$ | $10.7^{+4.8}_{-3.7}$ | 89.7 | 1.13 | 5944.5947 | 1.02 |
| 131 | 148.904062 | 69.077640 | 1.338 | 90 | 4.7 | $24.2^{+8.7}_{-7.7}$ | $31.9^{+6.8}_{-5.7}$ | $29.2^{+6.6}_{-5.5}$ | 89.7 | 2.20 | 5937.5945 | 1.87 |
| 132 | 148.851025 | 69.077614 | 1.563 | 77 | 3.2 | $11.0^{+8.3}_{-7.3}$ | $40.2^{+7.5}_{-6.4}$ | $22.6^{+6.0}_{-4.9}$ | 89.7 | 1.67 | 5940.5943 | 1.38 |
| 133 | 148.929932 | 69.079162 | 1.628 | 62 | 3.2 | $9.9^{+7.7}_{-6.6}$ | $32.3^{+6.8}_{-5.7}$ | $16.6^{+5.3}_{-4.2}$ | 89.9 | 1.97 | 5936.5941 | 1.74 |
| 134 | 148.972120 | 69.079687 | 2.250 | 22 | 2.8 | $17.4^{+5.8}_{-4.7}$ | $3.4^{+3.2}_{-1.9}$ | $-1.6^{+1.9}_{-nan}$ | 89.8 | 0.88 | 5941.5945 | 0.71 |
| 135 | 148.894383 | 69.081676 | 1.552 | 474 | 4.2 | $144.5^{+20.2}_{-19.1}$ | $219.0^{+15.9}_{-14.8}$ | $107.3^{+11.5}_{-10.4}$ | 90.0 | 5.02 | 5936.5942 | 4.43 |
| 136 | 148.684805 | 69.081713 | 4.716 | 109 | 10.0 | $10.4^{+9.4}_{-8.3}$ | $55.9^{+8.7}_{-7.6}$ | $32.7^{+7.3}_{-6.2}$ | 89.7 | 1.91 | 5935.5940 | 2.10 |
| 137 | 148.716858 | 69.082349 | 4.060 | 30 | 8.2 | $3.9^{+5.0}_{-3.8}$ | $8.1^{+4.3}_{-3.1}$ | $9.8^{+5.0}_{-3.8}$ | 90.0 | 1.15 | 5939.5949 | 1.07 |
| 138 | 148.906475 | 69.082757 | 1.648 | 124 | 3.9 | $35.6^{+10.5}_{-9.4}$ | $51.1^{+8.3}_{-7.2}$ | $34.4^{+7.1}_{-6.0}$ | 90.1 | 1.00 | 5940.5946 | 0.82 |
| 139 | 148.857191 | 69.082882 | 1.777 | 30 | 3.2 | $11.1^{+5.8}_{-4.7}$ | $9.2^{+4.3}_{-3.1}$ | $6.5^{+4.0}_{-2.8}$ | 89.3 | 1.80 | 5935.5945 | 1.77 |
| 140 | 148.792826 | 69.083983 | 2.694 | 3121 | 3.4 | $632.3^{+46.3}_{-45.3}$ | $1416.2^{+38.7}_{-37.6}$ | $1070.0^{+33.8}_{-32.7}$ | 89.7 | 7.83 | 5935.5943 | 6.33 |
| 141 | 148.842130 | 69.086266 | 2.104 | 1803 | 3.2 | $367.1^{+36.0}_{-35.0}$ | $856.3^{+30.3}_{-29.3}$ | $579.4^{+25.1}_{-24.1}$ | 89.6 | 5.94 | 5938.5943 | 4.79 |
| 142 | 148.962716 | 69.086746 | 2.406 | 53 | 3.5 | $12.2^{+7.2}_{-6.1}$ | $24.3^{+6.1}_{-5.0}$ | $13.1^{+5.0}_{-3.8}$ | 90.1 | 1.70 | 5939.5948 | 1.44 |
| 143 | 148.819301 | 69.086743 | 2.403 | 36 | 3.0 | $8.3^{+6.1}_{-5.0}$ | $15.3^{+5.1}_{-4.0}$ | $9.4^{+4.4}_{-3.3}$ | 89.2 | 1.24 | 5945.5947 | 1.04 |
| 144 | 148.886056 | 69.087086 | 1.877 | 22 | 3.2 | $19.0^{+5.8}_{-4.7}$ | $1.3^{+2.7}_{-1.3}$ | $-1.4^{+1.9}_{-nan}$ | 89.4 | 0.88 | 5935.5942 | 0.65 |
| 145 | 148.693505 | 69.087164 | 4.643 | 105 | 11.7 | $8.2^{+8.8}_{-7.7}$ | $47.3^{+8.1}_{-7.0}$ | $37.8^{+7.8}_{-6.7}$ | 89.6 | 1.43 | 5939.5949 | 1.42 |
| 146 | 148.983583 | 69.087508 | 2.745 | 36 | 3.9 | $4.3^{+5.9}_{-4.8}$ | $17.2^{+5.3}_{-4.2}$ | $10.6^{+4.7}_{-3.6}$ | 90.1 | 1.23 | 5937.5943 | 1.02 |
| 147 | 148.732856 | 69.088318 | 3.913 | 32 | 7.4 | $1.0^{+5.3}_{-4.2}$ | $14.5^{+5.1}_{-4.0}$ | $9.1^{+4.8}_{-3.7}$ | 89.7 | 1.25 | 5937.5946 | 1.14 |
| 148 | 148.841714 | 69.088648 | 2.229 | 64 | 1.2 | $23.7^{+8.2}_{-7.1}$ | $26.7^{+6.3}_{-5.2}$ | $12.4^{+4.7}_{-3.6}$ | 69.8 | 1.88 | 5937.5945 | 1.73 |
| 149 | 148.840996 | 69.089525 | 2.284 | 366 | 1.2 | $123.7^{+18.5}_{-17.5}$ | $180.7^{+14.5}_{-13.4}$ | $60.4^{+8.9}_{-7.8}$ | 69.2 | 5.41 | 5936.5940 | 4.40 |
| 150 | 148.861160 | 69.089956 | 2.144 | 33 | 3.6 | $-1.1^{+1.9}_{-nan}$ | $-0.8^{+1.9}_{-nan}$ | $31.2^{+6.8}_{-5.7}$ | 89.7 | 1.06 | 5935.5942 | 0.81 |
| 151 | 148.993925 | 69.090575 | 3.033 | 880 | 4.5 | $333.3^{+29.4}_{-28.3}$ | $468.0^{+22.7}_{-21.6}$ | $76.1^{+9.9}_{-8.9}$ | 90.3 | 2.89 | 5935.5944 | 2.42 |
| 152 | 148.957480 | 69.092219 | 2.604 | 5224 | 4.0 | $1042.1^{+59.4}_{-58.4}$ | $2362.1^{+49.6}_{-48.6}$ | $1821.7^{+43.7}_{-42.7}$ | 90.2 | 10.28 | 5939.5942 | 9.13 |
| 153 | 148.935777 | 69.092991 | 2.425 | 67 | 3.7 | $8.1^{+7.3}_{-6.2}$ | $29.2^{+6.5}_{-5.4}$ | $26.0^{+6.4}_{-5.3}$ | 89.8 | 1.26 | 5941.5943 | 1.03 |
| 154 | 148.945923 | 69.093384 | 2.539 | 31 | 3.9 | $2.1^{+5.2}_{-4.1}$ | $13.2^{+4.8}_{-3.7}$ | $11.8^{+4.8}_{-3.7}$ | 90.1 | 1.23 | 5940.5942 | 1.13 |
| 155 | 148.813322 | 69.093697 | 2.817 | 25 | 4.0 | $2.1^{+5.0}_{-3.8}$ | $11.2^{+4.6}_{-3.4}$ | $7.7^{+4.3}_{-3.1}$ | 89.9 | 1.34 | 5937.5943 | 1.27 |
| 156 | 148.705628 | 69.093929 | 4.586 | 39 | 12.3 | $-0.9^{+5.6}_{-4.4}$ | $16.6^{+5.4}_{-4.3}$ | $11.0^{+5.4}_{-4.3}$ | 89.7 | 1.35 | 5935.5946 | 1.35 |
| 157 | 148.958763 | 69.094644 | 2.741 | 30 | 4.2 | $7.2^{+5.7}_{-4.5}$ | $12.1^{+4.7}_{-3.6}$ | $6.5^{+4.1}_{-2.9}$ | 89.9 | 0.73 | 5947.5948 | 0.63 |
| 158 | 148.862338 | 69.095049 | 2.430 | 53 | 3.5 | $10.0^{+7.5}_{-6.4}$ | $29.3^{+6.5}_{-5.4}$ | $10.2^{+4.6}_{-3.4}$ | 89.5 | 1.28 | 5936.5937 | 1.06 |
| 159 | 149.011335 | 69.096485 | 3.547 | 45 | 3.4 | $1.5^{+6.3}_{-5.2}$ | $24.3^{+6.1}_{-5.0}$ | $15.8^{+5.3}_{-4.2}$ | 79.4 | 1.84 | 5938.5949 | 1.64 |
| 160 | 148.945840 | 69.097545 | 2.761 | 796 | 4.1 | $130.1^{+23.3}_{-22.3}$ | $366.1^{+20.2}_{-19.1}$ | $295.7^{+18.3}_{-17.3}$ | 89.8 | 4.32 | 5945.5947 | 3.30 |
| 161 | 148.932279 | 69.097610 | 2.655 | 23 | 4.0 | $-0.8^{+4.0}_{-2.8}$ | $7.2^{+4.0}_{-2.8}$ | $12.7^{+5.0}_{-3.8}$ | 90.0 | 1.40 | 5936.5942 | 1.37 |
| 162 | 148.897456 | 69.099343 | 2.612 | 66 | 3.9 | $6.1^{+7.3}_{-6.2}$ | $31.2^{+6.7}_{-5.6}$ | $24.8^{+6.3}_{-5.2}$ | 89.6 | 1.36 | 5944.5948 | 1.13 |
| 163 | 148.870092 | 69.103630 | 2.901 | 163 | 4.7 | $26.8^{+11.1}_{-10.1}$ | $73.1^{+9.6}_{-8.6}$ | $58.4^{+8.9}_{-7.8}$ | 90.6 | 2.01 | 5941.5943 | 2.31 |
| 164 | 148.996465 | 69.104881 | 3.708 | 236 | 6.7 | $67.0^{+14.7}_{-13.7}$ | $118.6^{+12.0}_{-10.9}$ | $43.8^{+8.0}_{-6.9}$ | 89.9 | 1.63 | 5935.5942 | 1.18 |
| 165 | 148.892020 | 69.105356 | 2.969 | 20 | 4.4 | $-0.0^{+4.1}_{-2.9}$ | $7.0^{+4.0}_{-2.8}$ | $8.6^{+4.4}_{-3.3}$ | 90.0 | 1.22 | 5935.5946 | 1.19 |
| 166 | 149.056483 | 69.108751 | 4.851 | 107 | 5.5 | $21.2^{+10.0}_{-8.9}$ | $57.1^{+8.7}_{-7.6}$ | $23.2^{+6.3}_{-5.2}$ | 89.8 | 2.92 | 5935.5942 | 2.62 |
| 167 | 148.902961 | 69.109179 | 3.209 | 147 | 3.0 | $28.4^{+11.3}_{-10.2}$ | $75.4^{+9.8}_{-8.7}$ | $41.2^{+7.6}_{-6.5}$ | 79.7 | 1.52 | 5945.5947 | 1.25 |
| 168 | 148.841184 | 69.110463 | 3.445 | 552 | 6.1 | $117.8^{+20.5}_{-19.5}$ | $259.8^{+17.2}_{-16.1}$ | $168.3^{+14.1}_{-13.1}$ | 89.5 | 3.86 | 5939.5946 | 2.79 |
| 169 | 148.897702 | 69.110629 | 3.289 | 144 | 3.4 | $26.3^{+10.9}_{-9.8}$ | $69.3^{+9.4}_{-8.3}$ | $45.0^{+7.9}_{-6.8}$ | 79.8 | 2.09 | 5939.5943 | 1.60 |
| 170 | 148.810390 | 69.111553 | 3.761 | 45 | 7.6 | $-0.3^{+4.7}_{-3.6}$ | $10.5^{+4.6}_{-3.4}$ | $27.2^{+6.7}_{-5.6}$ | 89.9 | 1.36 | 5938.5941 | 1.36 |
| 171 | 149.022500 | 69.112009 | 4.398 | 32 | 9.3 | $3.6^{+5.6}_{-4.4}$ | $13.0^{+5.0}_{-3.8}$ | $6.0^{+4.6}_{-3.4}$ | 89.7 | 1.12 | 5935.5940 | 1.05 |

TABLE 5 — *Continued*

| Src Num | RA (degrees) | Dec (degrees) | Avg OAA (arcmin) | Tot Src Counts | Tot Bkg Counts | Soft Net Counts | Medium Net Counts | Hard Net Counts | PSF % | Var Stat 5935-5949 | Var Obs 5935-5949 | Var Stat merged-735 |
|---|---|---|---|---|---|---|---|---|---|---|---|---|
| 172 | 148.926076 | 69.116704 | 3.726 | 33 | 7.5 | $21.6^{+6.4}_{-5.3}$ | $3.6^{+3.4}_{-2.2}$ | $0.3^{+3.4}_{-2.2}$ | 90.2 | 1.01 | 5946.5949 | 0.83 |
| 173 | 148.865520 | 69.117805 | 3.755 | 35 | 7.8 | $9.6^{+6.2}_{-5.1}$ | $13.6^{+5.0}_{-3.8}$ | $4.0^{+4.1}_{-2.9}$ | 90.5 | 1.31 | 5938.5945 | 1.12 |
| 174 | 148.891850 | 69.120344 | 3.868 | 102 | 8.8 | $16.4^{+8.7}_{-7.6}$ | $38.4^{+7.4}_{-6.3}$ | $38.4^{+7.7}_{-6.6}$ | 90.1 | 1.64 | 5940.5947 | 1.24 |
| 175 | 148.754293 | 69.124076 | 5.032 | 1562 | 17.6 | $39.4^{+28.3}_{-27.3}$ | $697.5^{+27.5}_{-26.5}$ | $807.5^{+29.6}_{-28.6}$ | 89.9 | 6.54 | 5936.5946 | 5.23 |
| 176 | 148.966010 | 69.127611 | 4.595 | 74 | 12.1 | $15.6^{+8.5}_{-7.5}$ | $36.7^{+7.3}_{-6.2}$ | $9.6^{+5.3}_{-4.2}$ | 89.9 | 2.05 | 5938.5949 | 1.81 |
| 177 | 148.790278 | 69.128677 | 4.872 | 251 | 16.1 | $39.1^{+13.5}_{-12.4}$ | $109.6^{+11.7}_{-10.6}$ | $87.2^{+10.9}_{-9.8}$ | 89.8 | 3.21 | 5941.5943 | 2.66 |
| 178 | 148.750227 | 69.129156 | 5.331 | 2102 | 22.5 | $461.7^{+39.0}_{-38.0}$ | $973.4^{+32.3}_{-31.3}$ | $644.3^{+26.7}_{-25.7}$ | 89.5 | 5.56 | 5935.5944 | 4.66 |
| 179 | 148.985373 | 69.134111 | 5.121 | 340 | 5.1 | $19.3^{+14.8}_{-13.7}$ | $168.0^{+14.0}_{-13.0}$ | $147.6^{+13.3}_{-12.3}$ | 59.6 | 2.34 | 5944.5945 | 1.81 |
| 180 | 148.955830 | 69.136574 | 5.037 | 1029 | 15.3 | $234.9^{+27.4}_{-26.4}$ | $455.0^{+22.4}_{-21.4}$ | $324.7^{+19.3}_{-18.3}$ | 89.7 | 7.02 | 5937.5942 | 6.24 |
| 181 | 148.790147 | 69.142269 | 5.615 | 193 | 25.6 | $36.0^{+12.0}_{-11.0}$ | $75.9^{+10.0}_{-9.0}$ | $56.5^{+9.6}_{-8.5}$ | 89.6 | 1.45 | 5937.5941 | 1.11 |
| 182 | 148.794173 | 69.145325 | 5.753 | 241 | 28.7 | $21.2^{+13.3}_{-12.2}$ | $118.6^{+12.2}_{-11.1}$ | $72.6^{+10.6}_{-9.5}$ | 89.8 | 1.61 | 5943.5944 | 1.37 |
| 183 | 148.851082 | 69.165904 | 6.655 | 4673 | 40.3 | $1056.1^{+55.6}_{-54.5}$ | $1905.4^{+44.7}_{-43.7}$ | $1679.2^{+42.3}_{-41.3}$ | 89.9 | 5.58 | 5941.5944 | 4.60 |
| 184 | 148.802999 | 69.028278 | 2.526 | 15 | 2.5 | $2.7^{+4.0}_{-2.8}$ | $4.5^{+3.4}_{-2.2}$ | $5.4^{+3.8}_{-2.6}$ | 89.6 | 0.87 | 5936.5937 | 0.78 |
| 185 | 148.799731 | 69.033411 | 2.380 | 12 | 2.8 | $0.6^{+3.4}_{-2.2}$ | $3.4^{+3.2}_{-1.9}$ | $5.2^{+3.8}_{-2.6}$ | 90.0 | 0.62 | 5935.5939 | 0.54 |
| 186 | 148.926060 | 69.084745 | 1.889 | 12 | 3.3 | $3.0^{+4.0}_{-2.8}$ | $3.3^{+3.2}_{-1.9}$ | $2.4^{+3.2}_{-1.9}$ | 89.6 | 0.64 | 5935.5948 | 0.57 |
| 187 | 148.745132 | 69.089350 | 3.719 | 24 | 6.5 | $2.1^{+4.6}_{-3.4}$ | $7.7^{+4.1}_{-2.9}$ | $7.8^{+4.6}_{-3.4}$ | 89.5 | 1.35 | 5937.5945 | 1.32 |
| 188 | 148.999880 | 69.092766 | 3.216 | 22 | 4.6 | $1.3^{+4.6}_{-3.4}$ | $9.0^{+4.3}_{-3.1}$ | $7.0^{+4.3}_{-3.1}$ | 89.8 | 0.99 | 5935.5947 | 0.92 |
| 189 | 149.052477 | 69.104124 | 4.584 | 22 | 6.2 | $3.2^{+4.6}_{-3.4}$ | $6.8^{+4.0}_{-2.8}$ | $5.9^{+4.3}_{-3.1}$ | 89.7 | 1.19 | 5940.5944 | 1.12 |
| 190 | 148.958689 | 69.120590 | 4.145 | 44 | 8.8 | $11.8^{+6.4}_{-5.3}$ | $13.4^{+5.0}_{-3.8}$ | $11.1^{+5.2}_{-4.1}$ | 89.8 | 1.31 | 5939.5948 | 1.07 |
| 191 | 148.974200 | 69.123340 | 4.424 | 22 | 10.3 | $0.7^{+5.0}_{-3.8}$ | $11.1^{+4.7}_{-3.6}$ | $-0.1^{+3.8}_{-2.6}$ | 89.8 | 0.96 | 5937.5945 | 0.90 |
| 192 | 149.016611 | 69.124346 | 4.945 | 24 | 10.7 | $1.5^{+5.1}_{-4.0}$ | $10.8^{+4.7}_{-3.6}$ | $0.9^{+4.0}_{-2.8}$ | 89.6 | 1.12 | 5935.5939 | 1.09 |
| 193 | 148.832026 | 69.125850 | 4.384 | 41 | 12.2 | $23.8^{+7.0}_{-5.9}$ | $6.7^{+4.1}_{-2.9}$ | $-1.7^{+3.6}_{-2.4}$ | 89.7 | 1.05 | 5947.5948 | 1.00 |
| 194 | 148.980538 | 69.137711 | 5.281 | 45 | 5.5 | $12.3^{+5.8}_{-4.7}$ | $8.0^{+4.1}_{-2.9}$ | $19.2^{+5.9}_{-4.8}$ | 59.7 | 1.61 | 5935.5942 | 1.57 |
| 195 | 148.839222 | 69.142114 | 5.291 | 74 | 21.4 | $37.2^{+9.1}_{-8.0}$ | $19.2^{+5.9}_{-4.8}$ | $-3.8^{+4.3}_{-3.1}$ | 89.6 | 1.30 | 5940.5946 | 1.14 |
| 196 | 148.982548 | 69.150299 | 6.020 | 41 | 20.3 | $0.1^{+5.5}_{-4.3}$ | $12.1^{+5.1}_{-4.0}$ | $8.6^{+5.8}_{-4.7}$ | 89.8 | 1.24 | 5935.5942 | 1.14 |
| 197 | 148.843674 | 69.043533 | 1.261 | 10 | 2.3 | $4.5^{+4.1}_{-2.9}$ | $3.5^{+3.2}_{-1.9}$ | $-0.2^{+2.3}_{-0.8}$ | 90.5 | 0.67 | 5935.5942 | 0.61 |
| 198 | 149.076907 | 69.052238 | 3.988 | 31 | 4.6 | $0.2^{+4.7}_{-3.6}$ | $11.1^{+4.6}_{-3.4}$ | $15.1^{+5.3}_{-4.2}$ | 89.8 | 1.60 | 5935.5937 | 1.59 |
| 199 | 148.697275 | 69.056138 | 4.157 | 26 | 7.8 | $13.0^{+5.4}_{-4.3}$ | $3.5^{+3.4}_{-2.2}$ | $1.7^{+3.8}_{-2.6}$ | 89.7 | 1.26 | 5940.5949 | 1.16 |
| 200 | 148.800948 | 69.062539 | 1.974 | 17 | 2.4 | $2.6^{+4.4}_{-3.3}$ | $7.5^{+4.0}_{-2.8}$ | $4.5^{+3.6}_{-2.4}$ | 89.6 | 0.66 | 5939.5944 | 0.50 |
| 201 | 148.781819 | 69.120508 | 4.527 | 33 | 13.2 | $3.7^{+5.2}_{-4.1}$ | $8.4^{+4.4}_{-3.3}$ | $7.7^{+5.1}_{-4.0}$ | 89.8 | 0.76 | 5935.5944 | 0.59 |
| 202 | 148.809220 | 69.128010 | 4.668 | 43 | 14.1 | $17.3^{+6.7}_{-5.6}$ | $9.1^{+4.6}_{-3.4}$ | $3.5^{+4.6}_{-3.4}$ | 90.0 | 1.05 | 5943.5944 | 1.08 |
| 203 | 149.024837 | 69.143037 | 6.019 | 76 | 14.1 | $14.2^{+8.2}_{-7.1}$ | $32.3^{+7.0}_{-5.9}$ | $15.4^{+6.1}_{-5.0}$ | 89.1 | 1.13 | 5936.5938 | 0.83 |
| 204 | 148.936284 | 69.167529 | 6.774 | 107 | 31.0 | $18.0^{+9.4}_{-8.3}$ | $40.9^{+7.9}_{-6.8}$ | $17.1^{+7.3}_{-6.2}$ | 90.1 | 1.89 | 5942.5947 | 1.36 |
| 205 | 149.012540 | 69.069204 | 2.723 | 13 | 3.7 | $2.4^{+3.4}_{-2.2}$ | $1.2^{+2.7}_{-1.3}$ | $5.7^{+4.0}_{-2.8}$ | 90.1 | 1.27 | 5936.5943 | 1.27 |
| 206 | 148.617612 | 69.098509 | 6.522 | 26 | 10.5 | $1.8^{+4.7}_{-3.6}$ | $7.8^{+4.3}_{-3.1}$ | $6.0^{+4.7}_{-3.6}$ | 90.5 | 0.98 | 5948.5949 | 0.86 |
| 207 | 148.981510 | 69.168578 | 7.059 | 50 | 18.5 | $1.2^{+6.4}_{-5.3}$ | $20.2^{+6.0}_{-4.9}$ | $10.1^{+5.8}_{-4.7}$ | 89.6 | 1.18 | 5938.5941 | 1.00 |
| 208 | 148.756936 | 69.177871 | 7.863 | 165 | 36.1 | $19.4^{+10.6}_{-9.6}$ | $60.8^{+9.2}_{-8.2}$ | $48.7^{+9.6}_{-8.6}$ | 90.0 | 1.97 | 5935.5945 | 1.54 |
| 209 | 148.694557 | 69.189989 | 9.087 | 167 | 49.3 | $14.1^{+10.4}_{-9.3}$ | $58.6^{+9.2}_{-8.1}$ | $45.1^{+10.0}_{-9.0}$ | 89.9 | 1.65 | 5941.5947 | 1.52 |
| 210 | 148.852091 | 69.247090 | 11.505 | 252 | 100.1 | $3.2^{+7.6}_{-6.5}$ | $3.6^{+5.9}_{-4.8}$ | $145.1^{+15.7}_{-14.7}$ | 90.3 | 5.13 | 5936.5944 | 5.06 |
| 211 | 148.650176 | 69.148875 | 7.625 | 77 | 24.2 | $9.2^{+8.1}_{-7.0}$ | $31.6^{+7.1}_{-6.0}$ | $12.0^{+6.4}_{-5.3}$ | 89.8 | 1.54 | 5941.5945 | 1.25 |
| 212 | 149.019621 | 69.200115 | 9.130 | 43 | 17.1 | $-0.7^{+6.0}_{-4.9}$ | $19.2^{+5.9}_{-4.8}$ | $7.4^{+5.5}_{-4.4}$ | 90.4 | 1.45 | 5935.5937 | 1.17 |
| 213 | 148.809932 | 69.209863 | 9.399 | 132 | 58.9 | $3.4^{+6.9}_{-5.8}$ | $14.5^{+6.0}_{-4.9}$ | $55.1^{+11.0}_{-10.0}$ | 90.1 | 1.72 | 5944.5945 | 1.37 |
| 214 | 149.038035 | 69.213380 | 10.011 | 86 | 21.8 | $10.4^{+8.5}_{-7.4}$ | $38.0^{+7.6}_{-6.5}$ | $15.8^{+6.7}_{-5.6}$ | 89.6 | 0.65 | 5936.5938 | 0.46 |

TABLE 5 — *Continued*

| Src Num | RA (degrees) | Dec (degrees) | Avg OAA (arcmin) | Tot Src Counts | Tot Bkg Counts | Soft Net Counts | Medium Net Counts | Hard Net Counts | PSF % | Var Stat 5935-5949 | Var Obs 5935-5949 | Var Stat merged-735 |
|---|---|---|---|---|---|---|---|---|---|---|---|---|
| 215 | 148.706666 | 69.194780 | 9.224 | 105 | 59.1 | $-1.1^{+6.7}_{-5.6}$ | $14.0^{+6.0}_{-4.9}$ | $33.0^{+9.7}_{-8.7}$ | 90.3 | 1.23 | 5943.5948 | 1.04 |
| 216 | 148.789441 | 69.194654 | 8.605 | 69 | 45.2 | $3.6^{+6.5}_{-5.4}$ | $11.7^{+5.6}_{-4.5}$ | $8.5^{+7.4}_{-6.4}$ | 90.2 | 1.02 | 5936.5944 | 1.02 |
| 217 | 148.755456 | 69.245517 | 11.741 | 297 | 154.5 | $17.4^{+13.0}_{-11.9}$ | $72.7^{+11.1}_{-10.0}$ | $52.4^{+14.0}_{-13.0}$ | 90.0 | 2.50 | 5942.5946 | 2.18 |
| 218 | 148.700678 | 69.256391 | 12.704 | 335 | 204.5 | $11.5^{+13.6}_{-12.6}$ | $80.2^{+11.9}_{-10.8}$ | $38.7^{+15.1}_{-14.1}$ | 90.4 | 1.42 | 5943.5945 | 1.06 |
| 219 | 148.911950 | 69.296395 | 14.449 | 269 | 132.8 | $-0.7^{+11.0}_{-10.0}$ | $52.2^{+9.9}_{-8.8}$ | $84.7^{+14.6}_{-13.5}$ | 90.4 | 1.83 | 5935.5939 | 1.39 |
| 220 | 148.524761 | 69.144328 | 9.594 | 53 | 8.1 | $0.2^{+6.5}_{-5.4}$ | $26.6^{+6.4}_{-5.3}$ | $18.0^{+6.0}_{-4.9}$ | 90.0 | 0.49 | 5947.5949 | 0.41 |
| 221 | 148.624136 | 69.172589 | 9.078 | 63 | 34.5 | $2.2^{+5.7}_{-4.6}$ | $8.3^{+4.9}_{-3.7}$ | $18.1^{+7.6}_{-6.5}$ | 90.1 | 0.84 | 5942.5945 | 0.76 |
| 222 | 148.618309 | 69.222821 | 11.618 | 151 | 106.1 | $22.9^{+9.3}_{-8.2}$ | $6.9^{+6.2}_{-5.1}$ | $15.1^{+10.6}_{-9.5}$ | 89.8 | 1.09 | 5939.5945 | 0.93 |
| 223 | 148.529750 | 69.238534 | 13.456 | 180 | 132.6 | $2.9^{+9.4}_{-8.3}$ | $28.1^{+8.2}_{-7.1}$ | $16.4^{+12.1}_{-11.1}$ | 90.3 | 2.16 | 5946.5949 | 1.87 |
| 224 | 148.688938 | 68.949751 | 7.608 | 67 | 5.9 | $26.4^{+8.9}_{-7.8}$ | $33.2^{+6.9}_{-5.8}$ | $1.5^{+3.6}_{-2.4}$ | 89.8 | 1.78 | 5935.5936 | 1.12 |
| 225 | 148.878180 | 69.062331 | 0.483 | 21 | 3.1 | $6.7^{+5.3}_{-4.2}$ | $9.0^{+4.3}_{-3.1}$ | $2.2^{+2.9}_{-1.6}$ | 69.7 | 1.63 | 5935.5938 | 1.61 |
| 226 | 149.197513 | 68.915061 | 10.656 | 308 | 75.6 | $18.0^{+13.8}_{-12.8}$ | $126.6^{+12.8}_{-11.8}$ | $87.8^{+13.3}_{-12.3}$ | 90.6 | 5.63 | 5945.5946 | 5.21 |
| 227 | 148.966806 | 69.026991 | 2.370 | 8 | 1.6 | $2.7^{+3.6}_{-2.4}$ | $2.7^{+2.9}_{-1.6}$ | $1.1^{+2.7}_{-1.3}$ | 89.8 | 0.91 | 5935.5947 | 0.90 |
| 228 | 148.552294 | 69.133681 | 8.748 | 23 | 8.5 | $1.2^{+4.1}_{-2.9}$ | $5.2^{+3.8}_{-2.6}$ | $8.1^{+4.9}_{-3.7}$ | 90.1 | 1.27 | 5947.5949 | 1.20 |
| 229 | 148.674860 | 69.045474 | 4.896 | 8 | 0.3 | $1.0^{+3.4}_{-2.2}$ | $3.9^{+3.2}_{-1.9}$ | $2.8^{+2.9}_{-1.6}$ | 89.7 | NA | NA | NA |
| 230 | 149.094076 | 69.079695 | 4.364 | 7 | 0.2 | $4.0^{+3.4}_{-2.2}$ | $1.0^{+2.3}_{-0.8}$ | $1.9^{+2.7}_{-1.3}$ | 90.0 | NA | NA | 0.00 |
| 231 | 148.665038 | 68.764394 | 18.110 | 334 | 328.7 | $4.8^{+11.4}_{-10.3}$ | $8.6^{+9.2}_{-8.2}$ | $-8.2^{+16.7}_{-15.7}$ | 90.2 | 3.05 | 5935.5936 | 2.28 |
| 232 | 148.633953 | 68.797864 | 16.382 | 45 | 36.4 | $1.4^{+4.5}_{-3.4}$ | $-0.1^{+3.5}_{-2.3}$ | $7.3^{+7.1}_{-6.0}$ | 90.5 | NA | NA | NA |
| 233 | 148.865943 | 68.834557 | 13.279 | 559 | 503.3 | $10.9^{+13.9}_{-12.9}$ | $30.6^{+11.3}_{-10.2}$ | $14.2^{+21.8}_{-20.7}$ | 89.9 | 2.00 | 5937.5940 | 1.71 |
| 234 | 148.605674 | 68.781450 | OC | OC | OC | OC | OC | OC | OC | OC | OC | OC |
| 235 | 148.674037 | 68.946622 | 7.937 | 10 | 2.9 | $2.6^{+4.0}_{-2.8}$ | $4.7^{+3.4}_{-2.2}$ | $-0.2^{+2.7}_{-1.3}$ | 90.2 | 0.41 | 5935.5936 | 0.28 |
| 236 | 148.787258 | 68.956596 | 6.326 | 21 | 9.7 | $8.9^{+5.1}_{-4.0}$ | $4.4^{+3.6}_{-2.4}$ | $-2.0^{+3.4}_{-2.2}$ | 89.7 | 1.12 | 5937.5940 | 1.07 |
| 237 | 148.813759 | 68.907238 | 9.047 | 35 | 32.9 | $-1.4^{+3.4}_{-2.2}$ | $-2.7^{+3.0}_{-1.7}$ | $6.2^{+6.6}_{-5.5}$ | 89.9 | 0.62 | 5936.5938 | 0.62 |
| 238 | 148.724725 | 68.915278 | 9.100 | 18 | 15.3 | $-1.5^{+3.6}_{-2.4}$ | $2.9^{+3.6}_{-2.4}$ | $1.3^{+4.6}_{-3.5}$ | 89.4 | 1.03 | 5935.5937 | 1.02 |
| 239 | 148.685333 | 68.936429 | 8.328 | 13 | 7.4 | $-0.0^{+3.2}_{-1.9}$ | $2.1^{+2.9}_{-1.6}$ | $3.5^{+4.1}_{-3.0}$ | 90.2 | 0.12 | 5935.5936 | 0.10 |
| 240 | 148.753090 | 68.942489 | 7.370 | 40 | 12.9 | $4.7^{+5.9}_{-4.8}$ | $15.2^{+5.2}_{-4.1}$ | $7.3^{+5.2}_{-4.1}$ | 90.0 | 1.40 | 5940.5941 | 1.20 |
| 241 | 148.638361 | 68.874879 | OC | OC | OC | OC | OC | OC | OC | OC | OC | OC |
| 242 | 148.667885 | 68.988036 | 6.140 | 1 | 0.1 | $-0.0^{+1.9}_{-nan}$ | $-0.0^{+1.9}_{-nan}$ | $0.9^{+2.3}_{-0.8}$ | 90.1 | NA | NA | NA |
| 243 | 148.715000 | 68.862399 | 12.159 | 170 | 153.4 | $6.9^{+9.0}_{-8.0}$ | $14.9^{+7.3}_{-6.3}$ | $-5.3^{+11.8}_{-10.8}$ | 90.3 | 0.80 | 5935.5936 | 0.59 |
| 244 | 148.817374 | 68.867299 | 11.403 | 287 | 245.1 | $11.7^{+10.7}_{-9.6}$ | $20.6^{+8.6}_{-7.6}$ | $9.6^{+15.6}_{-14.6}$ | 90.2 | 2.30 | 5938.5939 | 1.92 |
| 245 | 148.661261 | 68.878441 | 11.661 | 16 | 14.2 | $1.4^{+3.7}_{-2.4}$ | $1.2^{+3.0}_{-1.7}$ | $-0.8^{+4.4}_{-3.3}$ | 90.3 | NA | NA | NA |
| 246 | 148.696776 | 69.017169 | 4.623 | 2 | 1.5 | $-0.2^{+2.7}_{-1.3}$ | $1.7^{+2.7}_{-1.3}$ | $-1.1^{+1.9}_{-nan}$ | 90.5 | 0.48 | 5935.5937 | 0.48 |
| 247 | 148.913958 | 69.029801 | 1.649 | 3 | 1.6 | $0.7^{+2.3}_{-0.8}$ | $-0.4^{+1.9}_{-nan}$ | $1.0^{+2.7}_{-1.3}$ | 89.5 | 0.46 | 5935.5943 | 0.47 |
| 248 | 148.901714 | 69.044693 | 0.720 | 3 | 2.8 | $-1.0^{+2.7}_{-1.3}$ | $1.3^{+2.7}_{-1.3}$ | $-0.1^{+2.3}_{-0.8}$ | 90.3 | 0.37 | 5935.5942 | 0.40 |
| 249 | 148.928343 | 69.052188 | 0.832 | 2 | 3.0 | $-0.0^{+2.7}_{-1.3}$ | $0.3^{+2.3}_{-0.8}$ | $-1.3^{+1.9}_{-nan}$ | 90.6 | 0.64 | 5935.5941 | 0.65 |
| 250 | 148.894856 | 69.053795 | 0.184 | 6 | 4.3 | $-0.6^{+3.4}_{-2.2}$ | $2.8^{+3.2}_{-1.9}$ | $-0.5^{+2.3}_{-0.8}$ | 90.2 | 0.83 | 5935.5945 | 0.86 |
| 251 | 148.798452 | 69.055070 | 1.987 | 9 | 2.2 | $-0.3^{+1.9}_{-nan}$ | $-0.5^{+1.9}_{-nan}$ | $7.6^{+4.1}_{-2.9}$ | 89.5 | 0.63 | 5937.5943 | 0.59 |
| 252 | 148.891069 | 69.062112 | 0.390 | 22 | 10.1 | $1.9^{+5.4}_{-4.3}$ | $9.7^{+4.7}_{-3.6}$ | $0.3^{+2.9}_{-1.6}$ | 90.4 | 0.74 | 5935.5938 | 0.64 |
| 253 | 148.866498 | 69.068953 | 0.949 | 5 | 7.4 | $-1.1^{+2.9}_{-1.6}$ | $-1.2^{+2.3}_{-0.8}$ | $-0.1^{+2.7}_{-1.3}$ | 90.8 | 0.29 | 5935.5939 | 0.29 |
| 254 | 148.862479 | 69.070922 | 1.094 | 5 | 5.0 | $-1.8^{+2.3}_{-0.8}$ | $-0.3^{+2.3}_{-0.8}$ | $2.2^{+3.2}_{-1.9}$ | 90.3 | 0.56 | 5935.5947 | 0.59 |
| 255 | 148.859507 | 69.077017 | 1.440 | 4 | 3.8 | $1.8^{+2.9}_{-1.6}$ | $-1.0^{+1.9}_{-nan}$ | $-0.6^{+2.3}_{-0.8}$ | 89.8 | 0.36 | 5935.5938 | 0.38 |
| 256 | 148.980293 | 68.983117 | 4.772 | 18 | 7.0 | $1.9^{+4.4}_{-3.3}$ | $6.7^{+4.0}_{-2.8}$ | $2.4^{+3.8}_{-2.6}$ | 89.7 | 1.11 | 5935.5936 | 1.08 |
| 257 | 148.834595 | 69.031957 | 1.881 | 7 | 2.1 | $5.6^{+3.8}_{-2.6}$ | $0.5^{+2.3}_{-0.8}$ | $-0.3^{+2.3}_{-0.8}$ | 89.4 | 0.67 | 5936.5948 | 0.67 |
| 258 | 149.058756 | 69.040227 | 3.730 | 5 | 4.5 | $0.1^{+2.7}_{-1.3}$ | $0.2^{+2.3}_{-0.8}$ | $0.3^{+2.9}_{-1.6}$ | 89.9 | 0.41 | 5935.5941 | 0.41 |

TABLE 5 — *Continued*

| Src Num | RA (degrees) | Dec (degrees) | Avg OAA (arcmin) | Tot Src Counts | Tot Bkg Counts | Soft Net Counts | Medium Net Counts | Hard Net Counts | PSF % | Var Stat 5935-5949 | Var Obs 5935-5949 | Var Stat merged-735 |
|---|---|---|---|---|---|---|---|---|---|---|---|---|
| 259 | 148.780042 | 69.053969 | 2.384 | 12 | 2.9 | $6.6^{+4.4}_{-3.3}$ | $3.4^{+3.2}_{-1.9}$ | $-0.9^{+2.3}_{-0.8}$ | 90.0 | 0.74 | 5935.5942 | 0.74 |
| 260 | 148.985672 | 69.080494 | 2.511 | 8 | 3.2 | $-0.6^{+1.9}_{-nan}$ | $-0.7^{+1.9}_{-nan}$ | $6.1^{+4.0}_{-2.8}$ | 89.6 | 0.87 | 5935.5945 | 0.89 |
| 261 | 148.971470 | 69.088619 | 2.614 | 8 | 3.7 | $3.3^{+3.8}_{-2.6}$ | $2.2^{+2.9}_{-1.6}$ | $-1.1^{+2.3}_{-0.8}$ | 89.8 | 0.87 | 5936.5949 | 0.87 |
| 262 | 149.114785 | 69.169720 | OC | OC | OC | OC | OC | OC | OC | OC | OC | OC |
| 263 | 148.906620 | 69.054486 | 0.349 | 6 | 4.3 | $7.4^{+4.1}_{-2.9}$ | $-1.1^{+1.9}_{-nan}$ | $-1.5^{+1.9}_{-nan}$ | 90.3 | 0.35 | 5935.5939 | 0.33 |
| 264 | 148.885910 | 69.064708 | 0.552 | 990 | 20.9 | $195.7^{+26.5}_{-25.5}$ | $435.9^{+22.1}_{-21.0}$ | $337.5^{+19.5}_{-18.5}$ | 90.5 | 4.09 | 5935.5936 | 3.91 |
| 265 | 148.670052 | 69.096678 | 5.387 | 31 | 12.5 | $4.2^{+5.3}_{-4.2}$ | $9.5^{+4.6}_{-3.4}$ | $4.8^{+4.7}_{-3.6}$ | 89.5 | 1.02 | 5940.5946 | 0.88 |
| B1 | 149.289568 | 68.889505 | 13.090 | 392 | 335.2 | $8.3^{+10.1}_{-9.1}$ | $-6.8^{+7.9}_{-6.8}$ | $55.3^{+19.3}_{-18.3}$ | 90.4 | 1.59 | 5945.5947 | 1.46 |
| B2 | 148.899182 | 68.999208 | 3.409 | 9 | 3.6 | $-0.6^{+3.6}_{-2.4}$ | $5.2^{+3.6}_{-2.4}$ | $0.8^{+2.9}_{-1.6}$ | 90.2 | 0.69 | 5936.5939 | 0.61 |
| B3 | 148.928962 | 69.089610 | 2.182 | 15 | 3.3 | $0.2^{+3.4}_{-2.2}$ | $3.3^{+3.2}_{-1.9}$ | $8.2^{+4.3}_{-3.1}$ | 89.5 | 0.38 | 5936.5938 | 0.48 |
| B4 | 148.865808 | 69.108797 | 3.221 | 17 | 5.2 | $1.8^{+4.3}_{-3.1}$ | $6.0^{+3.8}_{-2.6}$ | $4.0^{+3.8}_{-2.6}$ | 89.8 | 1.17 | 5936.5946 | 1.06 |
| B5 | 148.867800 | 69.094913 | 2.395 | 13 | 3.5 | $4.0^{+4.1}_{-2.9}$ | $3.3^{+3.2}_{-1.9}$ | $2.2^{+3.2}_{-1.9}$ | 89.6 | 1.00 | 5936.5940 | 0.87 |
| B6 | 148.823682 | 68.995099 | 3.922 | 10 | 4.1 | $2.5^{+3.4}_{-2.2}$ | $1.3^{+2.7}_{-1.3}$ | $2.1^{+3.4}_{-2.2}$ | 89.9 | 1.18 | 5938.5947 | 2.43 |
| B7 | 148.697050 | 69.132804 | 6.218 | 45 | 30.0 | $-0.9^{+4.9}_{-3.7}$ | $5.4^{+4.4}_{-3.3}$ | $10.5^{+6.7}_{-5.6}$ | 89.6 | 1.05 | 5941.5944 | 1.01 |
| B8 | 148.582314 | 68.760019 | OC | OC | OC | OC | OC | OC | OC | OC | OC | OC |
| B9 | 148.657379 | 69.017001 | OC | OC | OC | OC | OC | OC | OC | OC | OC | OC |
| B10 | 148.781272 | 69.017103 | 3.334 | 7 | 3.7 | $-0.4^{+2.7}_{-1.3}$ | $1.4^{+2.7}_{-1.3}$ | $2.4^{+3.4}_{-2.2}$ | 89.9 | 0.70 | 5936.5943 | 0.70 |
| B11 | 148.776323 | 69.134773 | 5.333 | 32 | 20.5 | $-1.0^{+4.1}_{-3.0}$ | $2.9^{+3.8}_{-2.6}$ | $9.5^{+5.9}_{-4.8}$ | 89.4 | 1.06 | 5935.5940 | 1.12 |

NOTE. — Column 1: Source number. A "B" before the number refers to a borderline source not part of the master source list. Columns 2 & 3: Right ascension and Declination of the source in J2000 decimal degrees coordinates. Column 4: "Average OAA" = "Average Off-Axis Angle", the average angle on the sky between the source and the aimpoint of the observation in the merged observation. Column 5: "Tot Src Counts" refers to the number of source counts extracted in all of the source regions in observations 5935-5949. Column 6: "Tot Bkg Counts" refers to the number of background counts expected in the source region based on the nearby annular merged background extraction. Columns 7, 8 & 9: Soft (0.5-1 keV), Medium (1-2 keV), and Hard (2-8 keV) background-subracted counts with Gehrels (1986) errors. Column 10: "PSF %" is the average fraction of the point spread function enclosed by the source extraction region. Column 11: "Var Stat" is the variability statistic as defined in equation (1) between ObsIDs 5935-5949. Column 12: "Var Obs" are the two observations corresponding to column 11. Column 12: "Var Stat" is the variability statistic as defined in equation (1) between the merged observation and ObsID 735. Abbreviations of table values: "OC" = "Off Chip". "NA" = "Not Applicable/Available". This occurs in the case of the variability statistic when the source is only on the chips in one of ObsIDs 5935–5949 or off the ObsID 735 chips.

TABLE 6
MERGED FIT DATA OF SOURCES IN THE MASTER AND BORDERLINE SOURCE LISTS

| Src Num | Model Type | Γ or kT | Model Normalization | $N_H$ ($10^{22}$ cm$^{-2}$) | C-Stat (DOF) | Luminosity ($10^{37}$ erg s$^{-1}$) | Comments |
|---|---|---|---|---|---|---|---|
| 1 | plaw | $2.36^{+0.67}_{-0.56}$ | $4.35e\text{-}06^{+2.14e-06}_{-1.42e-06}$ | $0.14^{+0.14}_{-0.24}$ | 1231.6 (1014) | $1.92^{+0.41}_{-0.41}$ | |
| 2 | plaw | $1.29^{+0.39}_{-0.33}$ | $2.54e\text{-}06^{+9.80e-07}_{-6.34e-07}$ | $0.07^{+0.11}_{-0.07}$ | 1156.9 (1014) | $3.24^{+0.56}_{-0.56}$ | POC 5937, 5938 |
| 3 | plaw | $1.54^{+0.52}_{-0.44}$ | $3.62e\text{-}06^{+2.12e-06}_{-1.21e-06}$ | $0.27^{+0.20}_{-0.46}$ | 1073.4 (1014) | $3.08^{+0.57}_{-0.57}$ | POC 5939, 5940 |
| 4 | plaw | $2.53^{+3.01}_{-2.44}$ | $4.79e\text{-}06^{+1.38e-04}_{-4.53e-06}$ | $1.89^{+2.64}_{-1.89}$ | 1064.8 (1014) | $0.77^{+0.28}_{-0.28}$ | POC 5939, 5940 |
| 5 | plaw | $2.14^{+0.22}_{-0.21}$ | $2.31e\text{-}05^{+4.36e-06}_{-3.53e-06}$ | $0.16^{+0.06}_{-0.05}$ | 1127.9 (1014) | $11.61^{+0.65}_{-0.65}$ | |
| 6 | plaw | $1.65^{+0.75}_{-0.63}$ | $1.26e\text{-}05^{+1.11e-05}_{-5.54e-06}$ | $0.19^{+0.25}_{-0.19}$ | 1036.2 (1014) | $9.89^{+2.32}_{-2.32}$ | S61; POC 5937, 5938 |
| 7 | bbod | $0.80^{+0.27}_{-0.18}$ | $1.84e\text{-}07^{+9.48e-08}_{-6.03e-08}$ | $0.04^{+0.21}_{NA}$ | 1436.4 (1014) | $2.33^{+1.00}_{-1.00}$ | POC 5937, 5938, 5941–5946 |
| 8 | plaw | $1.89^{+0.58}_{-0.49}$ | $1.09e\text{-}05^{+5.20e-06}_{-3.32e-06}$ | $0.14^{+0.14}_{-0.26}$ | 1301.6 (1014) | $7.03^{+1.31}_{-1.31}$ | POC 5945 |
| 9 | bbod | $0.19^{+0.04}_{-0.01}$ | $1.91e\text{-}07^{+2.84e-08}_{-5.92e-08}$ | $0.04^{+0.02}_{NA}$ | 870.9 (1014) | $1.49^{+0.12}_{-0.12}$ | VC 41; POC 5935 |
| 10 | plaw | $1.22^{+0.37}_{-0.46}$ | $5.32e\text{-}07^{+1.58e-07}_{-1.98e-07}$ | $0.04^{+0.06}_{NA}$ | 756.3 (1014) | $0.75^{+0.24}_{-0.21}$ | S71 |
| 11 | plaw | $2.01^{+0.65}_{-0.52}$ | $1.16e\text{-}06^{+1.10e-06}_{-5.05e-07}$ | $0.53^{+0.39}_{-0.26}$ | 820.8 (1014) | $0.52^{+0.15}_{-0.13}$ | |
| 12 | plaw | $2.10^{+0.10}_{-0.22}$ | $8.02e\text{-}06^{+6.50e-07}_{-1.34e-06}$ | $0.04^{+0.02}_{-0.04}$ | 1041.0 (1014) | $4.90^{+0.21}_{-0.21}$ | S144 |
| 13 | plaw | $1.73^{+0.47}_{-0.46}$ | $2.25e\text{-}06^{+1.81e-06}_{-9.98e-07}$ | $1.07^{+0.44}_{-0.38}$ | 969.9 (1014) | $1.20^{+0.26}_{-0.23}$ | S162 |
| 14 | plaw | $1.71^{+0.38}_{-0.44}$ | $2.67e\text{-}06^{+1.99e-06}_{-1.16e-06}$ | $1.15^{+0.40}_{-0.39}$ | 907.9 (1014) | $1.44^{+0.28}_{-0.25}$ | S84 |
| 15 | plaw | $1.70^{f}_{f}$ | $4.40e\text{-}07^{+1.91e-07}_{-1.85e-07}$ | $0.04^{+0.01}_{NA}$ | 730.8 (1015) | $0.37^{+0.16}_{-0.13}$ | S62 |
| 16 | plaw | $2.21^{+0.28}_{-0.35}$ | $1.42e\text{-}06^{+3.01e-07}_{-3.24e-07}$ | $0.04^{+0.07}_{NA}$ | 956.7 (1014) | $0.80^{+0.15}_{-0.14}$ | S160 |
| 17 | plaw | $2.04^{+0.21}_{-0.19}$ | $4.54e\text{-}06^{+1.06e-06}_{-7.83e-07}$ | $0.12^{+0.07}_{-0.07}$ | 944.6 (1014) | $2.61^{+0.16}_{-0.16}$ | S136 |
| 18 | plaw | $1.79^{+0.11}_{-0.11}$ | $1.40e\text{-}05^{+1.81e-06}_{-1.61e-06}$ | $0.27^{+0.05}_{-0.05}$ | 1105.1 (1014) | $9.06^{+0.32}_{-0.32}$ | |
| 19 | plaw | $2.54^{+0.18}_{-0.18}$ | $1.95e\text{-}05^{+4.15e-06}_{-3.55e-06}$ | $0.72^{+0.10}_{-0.10}$ | 1067.4 (1014) | $4.45^{+0.21}_{-0.21}$ | S161 |
| 20 | plaw | $2.37^{+0.28}_{-0.25}$ | $1.23e\text{-}05^{+3.35e-06}_{-2.53e-06}$ | $0.17^{+0.09}_{-0.08}$ | 932.1 (1014) | $5.13^{+0.37}_{-0.37}$ | |
| 21 | plaw† | $1.85^{+0.02}_{-0.02}$ | $2.69e\text{-}04^{+6.64e-06}_{-6.50e-06}$ | $0.18^{+0.01}_{-0.01}$ | 1165.5 (1014) | $173.78^{+1.31}_{-1.31}$ | S105 |
| 22 | plaw | $2.35^{+0.17}_{-0.16}$ | $1.10e\text{-}05^{+1.88e-06}_{-1.53e-06}$ | $0.26^{+0.06}_{-0.06}$ | 1001.6 (1014) | $4.21^{+0.19}_{-0.19}$ | |
| 23 | bbod | $0.06^{+0.00}_{-0.01}$ | $1.02e\text{-}04^{+4.48e-04}_{-6.42e-05}$ | $0.42^{+0.13}_{-0.10}$ | 694.4 (1014) | $3.48^{+0.19}_{-0.19}$ | S171 |
| 24 | plaw | $1.85^{+0.67}_{-0.47}$ | $4.14e\text{-}07^{+3.22e-07}_{-1.20e-07}$ | $0.04^{+0.18}_{NA}$ | 809.3 (1014) | $0.31^{+0.10}_{-0.08}$ | S164 |
| 25 | plaw | $1.70^{f}_{f}$ | $2.84e\text{-}07^{+1.20e-07}_{-8.71e-08}$ | $0.11^{+0.18}_{NA}$ | 596.9 (1015) | $0.23^{+0.11}_{-0.09}$ | |
| 26 | plaw | $1.70^{f}_{f}$ | $3.09e\text{-}07^{+1.47e-07}_{-1.05e-07}$ | $0.67^{+0.45}_{-0.71}$ | 710.1 (1015) | $0.19^{+0.12}_{-0.09}$ | |
| 27 | plaw | $1.70^{f}_{f}$ | $2.39e\text{-}07^{+1.34e-07}_{-9.64e-08}$ | $0.64^{+0.63}_{-0.68}$ | 692.7 (1015) | $0.15^{+0.11}_{-0.08}$ | |
| 28 | plaw | $1.10^{+0.40}_{-0.40}$ | $7.85e\text{-}07^{+5.66e-07}_{-3.08e-07}$ | $0.32^{+0.30}_{-0.12}$ | 888.9 (1014) | $1.16^{+0.28}_{-0.24}$ | |
| 29 | plaw | $1.87^{+0.25}_{-0.23}$ | $4.35e\text{-}06^{+1.23e-06}_{-9.40e-07}$ | $0.22^{+0.11}_{-0.10}$ | 955.3 (1014) | $2.65^{+0.19}_{-0.19}$ | |
| 30 | plaw | $1.98^{+0.48}_{-0.45}$ | $1.68e\text{-}06^{+1.06e-06}_{-6.68e-07}$ | $0.48^{+0.26}_{-0.23}$ | 890.1 (1014) | $0.78^{+0.19}_{-0.17}$ | S166 |
| 31 | plaw | $2.02^{+0.65}_{-0.45}$ | $4.90e\text{-}07^{+3.03e-07}_{-1.41e-07}$ | $0.04^{+0.18}_{NA}$ | 688.6 (1014) | $0.32^{+0.11}_{-0.09}$ | |
| 32 | plaw | $1.11^{+0.81}_{-0.50}$ | $1.93e\text{-}07^{+2.30e-07}_{-7.44e-08}$ | $0.06^{+0.41}_{NA}$ | 723.8 (1014) | $0.31^{+0.13}_{-0.11}$ | |
| 33 | plaw | $1.70^{f}_{f}$ | $1.06e\text{-}05^{+2.09e-06}_{-1.76e-06}$ | $12.27^{+2.24}_{-1.97}$ | 939.3 (1015) | $2.62^{+0.55}_{-0.49}$ | S168 |
| 34 | plaw | $2.14^{+0.79}_{-0.75}$ | $1.10e\text{-}06^{+1.47e-06}_{-5.95e-07}$ | $0.48^{+0.51}_{-0.39}$ | 762.8 (1014) | $0.43^{+0.16}_{-0.13}$ | |
| 35 | plaw | $1.85^{+0.44}_{-0.41}$ | $2.74e\text{-}06^{+1.69e-06}_{-9.71e-07}$ | $0.34^{+0.24}_{-0.20}$ | 846.5 (1014) | $1.59^{+0.35}_{-0.31}$ | |
| 36 | plaw | $1.70^{f}_{f}$ | $9.96e\text{-}08^{+1.33e-06}_{NA}$ | $0.04^{NA}_{NA}$ | 750.8 (1015) | $0.08^{+0.06}_{-0.04}$ | S131 |
| 37 | plaw | $1.99^{+0.30}_{-0.28}$ | $1.12e\text{-}05^{+4.16e-06}_{-2.85e-06}$ | $0.40^{+0.15}_{-0.13}$ | 971.4 (1014) | $5.34^{+0.48}_{-0.48}$ | |
| 38 | bbod | $0.14^{+0.02}_{-0.03}$ | $2.41e\text{-}07^{+7.16e-07}_{-9.30e-08}$ | $0.04^{+0.20}_{NA}$ | 755.4 (1014) | $1.30^{+0.37}_{-0.32}$ | S60; VC 39 |
| 39 | bbod | $0.09^{+0.02}_{-0.01}$ | $2.31e\text{-}05^{+2.99e-04}_{-2.02e-05}$ | $0.57^{+0.25}_{-0.62}$ | 756.8 (1014) | $2.09^{+0.46}_{-0.41}$ | S56; VC 38; POC 5941 |
| 40 | plaw | $2.30^{+0.50}_{-0.42}$ | $2.27e\text{-}06^{+1.49e-06}_{-7.72e-07}$ | $0.32^{+0.23}_{-0.17}$ | 840.3 (1014) | $0.86^{+0.11}_{-0.11}$ | S125 |
| 41 | plaw | $1.34^{+0.35}_{-0.29}$ | $1.62e\text{-}06^{+7.67e-07}_{-4.29e-07}$ | $0.06^{+0.16}_{NA}$ | 879.7 (1014) | $1.97^{+0.21}_{-0.21}$ | POC 5935 |
| 42 | plaw | $1.98^{+0.65}_{-0.57}$ | $1.25e\text{-}06^{+1.46e-06}_{-5.94e-07}$ | $0.59^{+0.44}_{-0.34}$ | 881.2 (1014) | $0.56^{+0.15}_{-0.13}$ | |
| 43 | bbod | $0.19^{+0.05}_{-0.05}$ | $1.30e\text{-}08^{+3.99e-08}_{-5.08e-09}$ | $0.04^{+0.29}_{NA}$ | 718.0 (1014) | $0.10^{+0.06}_{-0.04}$ | S143 |
| 44 | plaw | $1.70^{f}_{f}$ | $1.27e\text{-}06^{+4.52e-07}_{-3.48e-07}$ | $3.59^{+1.47}_{-1.07}$ | 747.5 (1015) | $0.52^{+0.24}_{-0.19}$ | |
| 45 | plaw | $1.70^{f}_{f}$ | $7.79e\text{-}07^{+3.88e-07}_{-2.64e-07}$ | $0.26^{+0.40}_{-0.49}$ | 732.8 (1015) | $0.56^{+0.30}_{-0.23}$ | |
| 46 | plaw | $2.27^{+0.88}_{-0.62}$ | $3.92e\text{-}06^{+4.80e-06}_{-1.84e-06}$ | $0.40^{+0.37}_{-0.70}$ | 895.0 (1014) | $1.41^{+0.45}_{-0.41}$ | S65 |
| 47 | plaw | $2.43^{+0.77}_{-0.61}$ | $1.99e\text{-}06^{+1.55e-06}_{-7.80e-07}$ | $0.19^{+0.21}_{-0.40}$ | 950.8 (1014) | $0.78^{+0.13}_{-0.13}$ | S117; POC 5948 |
| 48 | plaw | $1.36^{+0.39}_{-0.31}$ | $7.41e\text{-}06^{+4.07e-06}_{-2.11e-06}$ | $0.09^{+0.21}_{-0.09}$ | 1000.9 (1014) | $8.58^{+0.81}_{-0.81}$ | |
| 49 | plaw | $1.83^{+1.09}_{-0.80}$ | $1.41e\text{-}06^{+4.34e-06}_{-8.85e-07}$ | $0.87^{+0.97}_{-0.50}$ | 855.6 (1014) | $0.69^{+0.31}_{-0.26}$ | POC 5939, 5940 |
| 50 | bbod | $0.06^{+0.01}_{-0.02}$ | $5.03e\text{-}04^{NA}_{-3.16e-04}$ | $1.30^{+0.91}_{-0.29}$ | 699.3 (1014) | $0.10^{+0.06}_{-0.05}$ | S142 |
| 51 | plaw | $1.70^{f}_{f}$ | $4.83e\text{-}07^{+1.74e-07}_{-1.34e-07}$ | $0.11^{+0.23}_{NA}$ | 816.2 (1015) | $0.38^{+0.17}_{-0.13}$ | POC 5941 |
| 52 | plaw | $1.76^{+0.86}_{-0.55}$ | $1.02e\text{-}06^{+1.22e-06}_{-4.41e-07}$ | $0.15^{+0.35}_{-0.15}$ | 952.9 (1014) | $0.73^{+0.25}_{-0.22}$ | VC 60 |
| 53 | plaw | $2.91^{+3.60}_{-2.22}$ | $5.14e\text{-}06^{+5.59e-04}_{-4.84e-06}$ | $3.65^{+6.45}_{-4.85}$ | 917.1 (1014) | $0.37^{+0.21}_{-0.18}$ | |
| 54 | plaw | $0.85^{+0.52}_{-0.43}$ | $4.34e\text{-}07^{+3.72e-07}_{-1.83e-07}$ | $0.15^{+0.32}_{NA}$ | 886.6 (1014) | $0.95^{+0.31}_{-0.27}$ | POC 5936 |
| 55 | plaw | $1.47^{+0.67}_{-0.72}$ | $1.22e\text{-}06^{+1.70e-06}_{-7.43e-07}$ | $0.67^{+0.66}_{-0.55}$ | 831.8 (1014) | $1.00^{+0.36}_{-0.31}$ | POC 5939, 5940 |
| 56 | plaw | $1.29^{+1.81}_{-0.78}$ | $5.80e\text{-}07^{+1.04e-06}_{-2.87e-07}$ | $0.04^{+0.61}_{NA}$ | 770.6 (1014) | $0.75^{+0.45}_{-0.37}$ | |
| 57 | plaw | $1.90^{+0.85}_{-0.79}$ | $1.89e\text{-}06^{+3.46e-06}_{-1.10e-06}$ | $0.68^{+0.70}_{-0.53}$ | 800.8 (1014) | $0.90^{+0.42}_{-0.34}$ | POC 5944 |

TABLE 6 — *Continued*

| Src Num | Model Type | Γ or kT | Model Normalization | $N_H$ ($10^{22}$ cm$^{-2}$) | C-Stat (DOF) | Luminosity ($10^{37}$ erg s$^{-1}$) | Comments |
|---|---|---|---|---|---|---|---|
| 58 | plaw | $1.70^{f}_{f}$ | 5.92e-07$^{+2.43e-07}_{-1.80e-07}$ | $0.07^{+0.20}_{NA}$ | 761.0 (1015) | $0.48^{+0.24}_{-0.19}$ | POC 5943 |
| 59 | plaw | $1.22^{+0.57}_{-0.53}$ | 2.36e-06$^{+2.40e-06}_{-1.04e-06}$ | $0.19^{+0.39}_{-0.19}$ | 804.2 (1014) | $3.08^{+1.09}_{-0.96}$ | S58 |
| 60 | plaw | $1.58^{+0.64}_{-0.46}$ | 8.18e-07$^{+6.39e-07}_{-2.56e-07}$ | $0.04^{+0.24}_{NA}$ | 880.8 (1014) | $0.78^{+0.34}_{-0.29}$ | S140; VC 52 |
| 61 | plaw | $1.11^{+0.61}_{-0.50}$ | 8.04e-07$^{+8.30e-07}_{-3.93e-07}$ | $0.25^{+0.42}_{-0.25}$ | 1010.5 (1014) | $1.19^{+0.30}_{-0.30}$ | POC 5935 |
| 62 | 3mods‡ | $NA^{NA}_{NA}$ | $NA^{NA}_{NA}$ | $NA^{NA}_{NA}$ | 941.1 (1012) | $20.82^{+0.36}_{-0.36}$ | S88 |
| 63 | plaw | $1.21^{+0.30}_{-0.35}$ | 4.29e-07$^{+1.42e-07}_{-1.22e-07}$ | $0.04^{+0.09}_{NA}$ | 840.6 (1014) | $0.61^{+0.16}_{-0.14}$ | S72 |
| 64 | plaw | $1.70^{f}_{f}$ | 5.04e-07$^{+2.97e-07}_{-1.99e-07}$ | $4.18^{+2.28}_{-1.61}$ | 659.6 (1015) | $0.19^{+0.15}_{-0.11}$ | |
| 65 | plaw | $0.56^{+0.55}_{-0.45}$ | 4.22e-07$^{+5.21e-07}_{-1.94e-07}$ | $0.56^{+0.61}_{-0.42}$ | 914.4 (1014) | $1.31^{+0.30}_{-0.26}$ | S54 |
| 66 | plaw | $2.21^{+0.48}_{-0.43}$ | 2.07e-06$^{+1.26e-06}_{-7.48e-07}$ | $0.50^{+0.21}_{-0.18}$ | 826.9 (1014) | $0.75^{+0.16}_{-0.14}$ | S150 |
| 67 | plaw | $2.33^{+4.03}_{-0.61}$ | 2.86e-07$^{+4.47e-07}_{-8.38e-08}$ | $0.04^{+1.15}_{NA}$ | 683.9 (1014) | $0.15^{+0.05}_{-0.04}$ | S127 |
| 68 | plaw | $1.79^{+0.50}_{-0.46}$ | 8.32e-07$^{+5.77e-07}_{-3.17e-07}$ | $0.31^{+0.23}_{-0.19}$ | 744.3 (1014) | $0.52^{+0.14}_{-0.12}$ | S163 |
| 69 | plaw | $1.70^{f}_{f}$ | 4.57e-07$^{+2.16e-07}_{-1.54e-07}$ | $2.13^{+0.99}_{-0.76}$ | 692.0 (1015) | $0.22^{+0.12}_{-0.09}$ | |
| 70 | plaw | $1.70^{f}_{f}$ | 2.61e-07$^{+8.80e-08}_{-6.77e-08}$ | $0.29^{+0.19}_{-0.30}$ | 636.9 (1015) | $0.18^{+0.08}_{-0.06}$ | |
| 71 | plaw | $0.27^{+0.62}_{-0.50}$ | 1.15e-07$^{+1.29e-07}_{-5.56e-08}$ | $0.19^{+0.49}_{NA}$ | 780.7 (1014) | $0.59^{+0.20}_{-0.16}$ | |
| 72 | plaw | $1.87^{+0.28}_{-0.29}$ | 2.39e-06$^{+8.88e-07}_{-6.48e-07}$ | $0.55^{+0.15}_{-0.14}$ | 877.7 (1014) | $1.23^{+0.11}_{-0.11}$ | S104 |
| 73 | plaw | $1.65^{+0.23}_{-0.28}$ | 1.04e-06$^{+2.34e-07}_{-2.22e-07}$ | $0.04^{+0.06}_{NA}$ | 887.1 (1014) | $0.93^{+0.09}_{-0.09}$ | S152 |
| 74 | plaw | $1.89^{+0.71}_{-0.61}$ | 5.23e-06$^{+4.63e-06}_{-2.39e-06}$ | $0.19^{+0.23}_{-0.19}$ | 989.2 (1014) | $3.21^{+0.16}_{-0.16}$ | S51; RS 5945 |
| 75 | bbod | $0.07^{+0.02}_{-0.01}$ | 7.96e-07$^{+1.67e-05}_{-6.89e-07}$ | $0.17^{+0.25}_{-0.17}$ | 599.6 (1014) | $0.28^{+0.06}_{-0.05}$ | S96 |
| 76 | plaw | $1.70^{f}_{f}$ | 1.59e-07$^{+5.05e-08}_{-6.22e-08}$ | $0.04^{+0.02}_{NA}$ | 658.9 (1015) | $0.13^{+0.06}_{-0.05}$ | S122 |
| 77 | plaw | $1.66^{+0.52}_{-0.36}$ | 3.48e-07$^{+1.88e-07}_{-9.32e-08}$ | $0.04^{+0.15}_{NA}$ | 753.1 (1014) | $0.31^{+0.09}_{-0.07}$ | S101 |
| 78 | plaw | $1.89^{+0.17}_{-0.17}$ | 4.48e-06$^{+8.18e-07}_{-6.89e-07}$ | $0.23^{+0.06}_{-0.06}$ | 927.2 (1014) | $2.68^{+0.14}_{-0.14}$ | S93 |
| 79 | plaw | $1.86^{+0.30}_{-0.29}$ | 1.89e-06$^{+6.32e-07}_{-4.70e-07}$ | $0.18^{+0.11}_{-0.10}$ | 930.8 (1014) | $1.20^{+0.11}_{-0.11}$ | S175 |
| 80 | plaw | $1.74^{+0.19}_{-0.19}$ | 3.19e-06$^{+6.73e-07}_{-5.38e-07}$ | $0.19^{+0.07}_{-0.06}$ | 980.0 (1014) | $2.28^{+0.13}_{-0.13}$ | S111 |
| 81 | bbod | $0.10^{+0.05}_{-0.03}$ | 1.97e-07$^{+2.16e-05}_{-1.20e-07}$ | $0.44^{+0.50}_{-0.34}$ | 743.0 (1014) | $0.06^{+0.03}_{-0.02}$ | |
| 82 | plaw | $1.70^{f}_{f}$ | 1.83e-07$^{+7.67e-08}_{-5.66e-08}$ | $0.21^{+0.24}_{-0.32}$ | 702.8 (1015) | $0.13^{+0.06}_{-0.05}$ | |
| 83 | plaw | $1.70^{f}_{f}$ | 2.26e-07$^{+1.11e-07}_{-7.55e-08}$ | $0.54^{+0.45}_{-0.58}$ | 724.3 (1015) | $0.14^{+0.08}_{-0.06}$ | |
| 84 | plaw | $1.73^{+0.18}_{-0.18}$ | 2.96e-06$^{+5.48e-07}_{-4.59e-07}$ | $0.12^{+0.06}_{-0.06}$ | 963.0 (1014) | $2.26^{+0.13}_{-0.13}$ | S139 |
| 85 | plaw | $1.70^{f}_{f}$ | 1.42e-07$^{+7.25e-08}_{-5.19e-08}$ | $0.30^{+0.36}_{-0.45}$ | 647.0 (1015) | $0.10^{+0.06}_{-0.04}$ | |
| 86 | plaw | $1.50^{+0.07}_{-0.07}$ | 1.68e-05$^{+1.24e-06}_{-1.15e-06}$ | $0.10^{+0.02}_{-0.02}$ | 1060.8 (1014) | $16.64^{+0.38}_{-0.38}$ | |
| 87 | bbod | $0.15^{+0.03}_{-0.02}$ | 3.61e-08$^{+2.91e-08}_{-1.32e-08}$ | $0.04^{+0.09}_{NA}$ | 851.3 (1014) | $0.21^{+0.05}_{-0.04}$ | S155 |
| 88 | plaw | $1.70^{f}_{f}$ | 1.47e-07$^{+4.09e-08}_{-4.95e-08}$ | $0.04^{+0.06}_{NA}$ | 637.4 (1015) | $0.12^{+0.06}_{-0.05}$ | |
| 89 | plaw | $1.45^{+0.34}_{-0.48}$ | 2.59e-07$^{+8.09e-08}_{-8.74e-08}$ | $0.04^{+0.07}_{NA}$ | 770.6 (1014) | $0.28^{+0.09}_{-0.08}$ | |
| 90 | plaw | $1.85^{+0.11}_{-0.11}$ | 8.95e-06$^{+1.01e-06}_{-9.08e-07}$ | $0.16^{+0.04}_{-0.04}$ | 970.9 (1014) | $5.84^{+0.20}_{-0.20}$ | S118 |
| 91 | plaw | $1.97^{+0.31}_{-0.28}$ | 1.60e-06$^{+4.92e-07}_{-3.69e-07}$ | $0.15^{+0.09}_{-0.09}$ | 784.8 (1014) | $0.95^{+0.08}_{-0.08}$ | S100 |
| 92 | plaw | $1.62^{+0.16}_{-0.23}$ | 2.11e-06$^{+3.28e-07}_{-3.83e-07}$ | $0.04^{+0.04}_{NA}$ | 909.1 (1014) | $1.93^{+0.12}_{-0.12}$ | |
| 93 | plaw | $1.69^{+0.24}_{-0.32}$ | 7.38e-07$^{+1.66e-07}_{-1.74e-07}$ | $0.04^{+0.06}_{NA}$ | 789.0 (1014) | $0.63^{+0.12}_{-0.11}$ | S98 |
| 94 | plaw | $1.43^{+0.30}_{-0.30}$ | 1.03e-06$^{+4.00e-07}_{-2.74e-07}$ | $0.19^{+0.12}_{-0.11}$ | 849.5 (1014) | $1.05^{+0.11}_{-0.11}$ | S170 |
| 95 | plaw | $2.66^{+0.63}_{-0.81}$ | 2.30e-07$^{+6.55e-08}_{-8.23e-08}$ | $0.04^{+0.06}_{NA}$ | 728.6 (1014) | $0.10^{+0.04}_{-0.04}$ | |
| 96 | bbod | $0.09^{+0.01}_{-0.00}$ | 3.63e-06$^{+2.86e-07}_{-1.52e-06}$ | $0.04^{+0.01}_{-0.04}$ | 811.9 (1014) | $7.41^{+0.17}_{-0.17}$ | S132 |
| 97 | plaw | $1.05^{+0.21}_{-0.37}$ | 4.37e-07$^{+8.75e-08}_{-1.35e-07}$ | $0.04^{+0.04}_{NA}$ | 804.0 (1014) | $0.76^{+0.17}_{-0.15}$ | S110 |
| 98 | plaw | $1.53^{+0.40}_{-0.34}$ | 1.27e-06$^{+7.53e-07}_{-4.21e-07}$ | $0.42^{+0.24}_{-0.19}$ | 894.8 (1014) | $1.03^{+0.20}_{-0.18}$ | S176; RS 5935 |
| 99 | bbod | $0.43^{+0.09}_{-0.07}$ | 1.38e-08$^{+4.95e-09}_{-3.30e-09}$ | $0.04^{+0.18}_{NA}$ | 655.1 (1014) | $0.16^{+0.06}_{-0.05}$ | VC 225 |
| 100 | plaw | $1.50^{+0.07}_{-0.07}$ | 1.73e-05$^{+1.38e-06}_{-1.25e-06}$ | $0.19^{+0.03}_{-0.03}$ | 1043.9 (1014) | $16.13^{+0.39}_{-0.39}$ | S116 |
| 101 | plaw | $1.24^{+0.47}_{-0.42}$ | 3.49e-07$^{+2.25e-07}_{-1.30e-07}$ | $0.13^{+0.18}_{-0.13}$ | 713.7 (1014) | $0.46^{+0.12}_{-0.11}$ | S80; RS 5939, 5940 |
| 102 | plaw | $2.63^{+0.72}_{-0.61}$ | 5.80e-07$^{+4.04e-07}_{-2.11e-07}$ | $0.17^{+0.17}_{-0.36}$ | 621.5 (1014) | $0.21^{+0.06}_{-0.05}$ | RS 5935 |
| 103 | plaw | $2.10^{+0.45}_{-0.38}$ | 9.40e-07$^{+4.06e-07}_{-2.66e-07}$ | $0.08^{+0.11}_{-0.08}$ | 756.5 (1014) | $0.54^{+0.06}_{-0.06}$ | |
| 104 | plaw | $1.70^{f}_{f}$ | 5.87e-07$^{+2.20e-07}_{-1.66e-07}$ | $1.67^{+0.74}_{-0.54}$ | 665.1 (1015) | $0.29^{+0.14}_{-0.11}$ | RS 735 |
| 105 | plaw | $1.74^{+0.15}_{-0.16}$ | 4.81e-06$^{+7.36e-07}_{-6.67e-07}$ | $0.08^{+0.04}_{-0.04}$ | 884.4 (1014) | $3.78^{+0.18}_{-0.18}$ | S109; VC 106 |
| 106 | plaw | $0.58^{+0.10}_{-0.25}$ | 1.95e-06$^{+1.85e-07}_{-4.79e-07}$ | $0.04^{+0.01}_{NA}$ | 1072.3 (1014) | $6.48^{+0.34}_{-0.34}$ | S112; VC 105 |
| 107 | plaw | $1.70^{f}_{f}$ | 6.21e-07$^{+2.52e-07}_{-1.96e-07}$ | $2.22^{+0.99}_{-0.84}$ | 660.1 (1015) | $0.29^{+0.13}_{-0.10}$ | S79 |
| 108 | plaw | $1.69^{+0.13}_{-0.12}$ | 6.12e-06$^{+8.03e-07}_{-6.81e-07}$ | $0.09^{+0.04}_{-0.04}$ | 946.4 (1014) | $4.95^{+0.20}_{-0.20}$ | S120; RS 735 |
| 109 | plaw | $1.81^{+0.72}_{-0.46}$ | 2.67e-07$^{+1.79e-07}_{-8.12e-08}$ | $0.04^{+0.19}_{NA}$ | 726.1 (1014) | $0.20^{+0.07}_{-0.06}$ | |
| 110 | plaw | $1.70^{f}_{f}$ | 1.84e-07$^{+4.86e-08}_{-5.21e-08}$ | $0.04^{+0.07}_{NA}$ | 629.2 (1015) | $0.16^{+0.07}_{-0.05}$ | |
| 111 | plaw | $1.84^{+0.27}_{-0.24}$ | 1.67e-06$^{+4.76e-07}_{-3.39e-07}$ | $0.12^{+0.08}_{-0.07}$ | 832.7 (1014) | $1.15^{+0.09}_{-0.09}$ | RS 735 |
| 112 | plaw | $1.75^{+0.53}_{-0.45}$ | 5.38e-07$^{+3.27e-07}_{-1.87e-07}$ | $0.17^{+0.17}_{-0.14}$ | 756.7 (1014) | $0.39^{+0.10}_{-0.09}$ | S90; RS 735 |
| 113 | plaw | $1.54^{+0.35}_{-0.32}$ | 8.03e-07$^{+3.15e-07}_{-2.28e-07}$ | $0.10^{+0.12}_{-0.10}$ | 791.5 (1014) | $0.76^{+0.09}_{-0.09}$ | |
| 114 | plaw | $2.19^{+0.35}_{-0.32}$ | 1.35e-06$^{+4.48e-07}_{-3.26e-07}$ | $0.13^{+0.10}_{-0.09}$ | 801.1 (1014) | $0.67^{+0.07}_{-0.07}$ | S63; RS 5935 |
| 115 | bbod | $0.36^{+0.12}_{-0.08}$ | 9.22e-09$^{+5.75e-09}_{-2.54e-09}$ | $0.04^{+0.25}_{NA}$ | 673.3 (1014) | $0.10^{+0.04}_{-0.04}$ | |

TABLE 6 — *Continued*

| Src Num | Model Type | Γ or kT | Model Normalization | $N_H$ ($10^{22}$ cm$^{-2}$) | C-Stat (DOF) | Luminosity ($10^{37}$ erg s$^{-1}$) | Comments |
|---|---|---|---|---|---|---|---|
| 116 | plaw | $2.24^{+0.28}_{-0.26}$ | 3.24e-06$^{+9.62e-07}_{-7.02e-07}$ | $0.36^{+0.10}_{-0.09}$ | 838.8 (1014) | $1.24^{+0.09}_{-0.09}$ | S67 |
| 117 | plaw | $1.45^{+0.17}_{-0.15}$ | 2.96e-06$^{+5.24e-07}_{-4.09e-07}$ | $0.07^{+0.05}_{-0.05}$ | 967.8 (1014) | $3.15^{+0.17}_{-0.17}$ | S115 |
| 118 | plaw | $1.70^{f}_{f}$ | 1.64e-07$^{+7.10e-08}_{-5.25e-08}$ | $0.20^{+0.20}_{-0.31}$ | 659.6 (1015) | $0.12^{+0.06}_{-0.05}$ | |
| 119 | bbod | $0.45^{+0.07}_{-0.06}$ | 3.36e-08$^{+8.52e-09}_{-6.25e-09}$ | $0.21^{+0.17}_{-0.14}$ | 738.5 (1014) | $0.33^{+0.07}_{-0.07}$ | |
| 120 | bbod | $0.07^{+0.02}_{-0.02}$ | 1.07e-05$^{+3.11e-02}_{-1.03e-05}$ | $0.77^{+0.41}_{-0.79}$ | 629.1 (1014) | $0.13^{+0.04}_{-0.03}$ | RS 5939, 5940 |
| 121 | plaw | $1.81^{+0.14}_{-0.14}$ | 6.20e-06$^{+8.65e-07}_{-7.96e-07}$ | $0.18^{+0.04}_{-0.04}$ | 942.7 (1014) | $4.16^{+0.18}_{-0.18}$ | S102; two sources? |
| 122 | plaw | $2.16^{+0.91}_{-0.70}$ | 3.89e-07$^{+4.64e-07}_{-2.04e-07}$ | $0.29^{+0.29}_{-0.22}$ | 741.2 (1014) | $0.17^{+0.07}_{-0.06}$ | S48 |
| 123 | plaw | $1.84^{+0.68}_{-0.54}$ | 7.26e-07$^{+8.18e-07}_{-3.25e-07}$ | $0.62^{+0.44}_{-0.29}$ | 789.0 (1014) | $0.38^{+0.12}_{-0.10}$ | |
| 124 | plaw | $1.70^{f}_{f}$ | 2.74e-07$^{+1.09e-07}_{-8.31e-08}$ | $0.51^{+0.38}_{-0.52}$ | 666.8 (1015) | $0.18^{+0.09}_{-0.07}$ | |
| 125 | bbod | $1.09^{+0.38}_{-0.25}$ | 3.44e-07$^{+2.49e-07}_{-9.31e-08}$ | $14.27^{+5.93}_{-4.60}$ | 846.6 (1014) | $1.42^{+0.36}_{-0.31}$ | S135; RS 5946, 5947 |
| 126 | plaw | $2.09^{+0.16}_{-0.16}$ | 5.70e-06$^{+9.07e-07}_{-7.69e-07}$ | $0.18^{+0.05}_{-0.05}$ | 941.2 (1014) | $2.92^{+0.14}_{-0.14}$ | S126 |
| 127 | plaw | $1.92^{+0.29}_{-0.25}$ | 1.82e-06$^{+5.44e-07}_{-3.90e-07}$ | $0.19^{+0.09}_{-0.08}$ | 846.9 (1014) | $1.08^{+0.09}_{-0.09}$ | S151; RS 5944 |
| 128 | plaw | $2.81^{+0.17}_{-0.16}$ | 1.28e-05$^{+1.75e-06}_{-1.51e-06}$ | $0.26^{+0.04}_{-0.04}$ | 943.4 (1014) | $3.56^{+0.14}_{-0.14}$ | RS 5943 |
| 129 | plaw | $1.66^{+0.58}_{-0.49}$ | 5.08e-07$^{+4.04e-07}_{-2.07e-07}$ | $0.34^{+0.24}_{-0.20}$ | 762.7 (1014) | $0.37^{+0.12}_{-0.10}$ | S53 |
| 130 | bbod | $0.45^{+0.13}_{-0.11}$ | 4.11e-08$^{+5.47e-08}_{-1.67e-08}$ | $1.57^{+0.94}_{-0.68}$ | 785.1 (1014) | $0.19^{+0.07}_{-0.06}$ | |
| 131 | plaw | $1.47^{+0.26}_{-0.30}$ | 6.51e-07$^{+1.78e-07}_{-1.53e-07}$ | $0.04^{+0.08}_{NA}$ | 831.3 (1014) | $0.69^{+0.13}_{-0.12}$ | |
| 132 | plaw | $1.93^{+0.43}_{-0.37}$ | 1.10e-06$^{+5.84e-07}_{-3.41e-07}$ | $0.34^{+0.17}_{-0.14}$ | 814.9 (1014) | $0.58^{+0.12}_{-0.11}$ | S85 |
| 133 | plaw | $2.20^{+0.55}_{-0.45}$ | 8.65e-07$^{+5.48e-07}_{-3.01e-07}$ | $0.26^{+0.17}_{-0.14}$ | 727.5 (1014) | $0.38^{+0.09}_{-0.08}$ | S134 |
| 134 | bbod | $0.11^{+0.03}_{-0.03}$ | 3.58e-08$^{+6.54e-07}_{-2.39e-08}$ | $0.09^{+0.31}_{-0.09}$ | 580.5 (1014) | $0.08^{+0.04}_{-0.03}$ | |
| 135 | plaw | $1.97^{+0.95}_{-0.68}$ | 4.83e-06$^{+5.72e-06}_{-2.13e-06}$ | $0.11^{+0.26}_{-0.11}$ | 963.3 (1014) | $2.99^{+0.14}_{-0.14}$ | S113 |
| 136 | plaw | $2.36^{+0.63}_{-0.54}$ | 3.07e-06$^{+2.77e-06}_{-1.24e-06}$ | $0.56^{+0.31}_{-0.24}$ | 798.6 (1014) | $0.92^{+0.10}_{-0.10}$ | POC 5935, 5936, 735 |
| 137 | plaw | $1.89^{+1.13}_{-0.90}$ | 3.30e-07$^{+4.91e-07}_{-1.87e-07}$ | $0.36^{+0.39}_{-0.30}$ | 772.1 (1014) | $0.18^{+0.08}_{-0.07}$ | |
| 138 | plaw | $1.49^{+1.29}_{-0.75}$ | 9.10e-07$^{+1.86e-06}_{-4.37e-07}$ | $0.04^{+0.39}_{NA}$ | 873.3 (1014) | $0.95^{+0.09}_{-0.09}$ | S128 |
| 139 | plaw | $1.97^{+0.44}_{-0.57}$ | 2.48e-07$^{+8.22e-08}_{-8.14e-08}$ | $0.04^{+0.07}_{NA}$ | 730.0 (1014) | $0.17^{+0.06}_{-0.05}$ | |
| 140 | plaw | $1.39^{+0.35}_{-0.20}$ | 2.71e-05$^{+1.40e-05}_{-7.47e-06}$ | $0.11^{+0.08}_{-0.06}$ | 1180.2 (1014) | $30.10^{+0.54}_{-0.54}$ | S69 |
| 141 | plaw | $1.56^{+0.07}_{-0.07}$ | 1.70e-05$^{+1.35e-06}_{-1.18e-06}$ | $0.15^{+0.03}_{-0.02}$ | 1109.6 (1014) | $15.21^{+0.36}_{-0.36}$ | S83 |
| 142 | plaw | $2.18^{+0.53}_{-0.51}$ | 7.11e-07$^{+4.14e-07}_{-2.64e-07}$ | $0.23^{+0.16}_{-0.15}$ | 735.8 (1014) | $0.32^{+0.08}_{-0.07}$ | |
| 143 | plaw | $1.46^{+3.86}_{-1.60}$ | 3.10e-07$^{NA}_{NA}$ | $0.11^{NA}_{NA}$ | 866.5 (1014) | $0.32^{+0.10}_{-0.09}$ | |
| 144 | plaw | $1.70^{f}_{f}$ | 1.58e-07$^{+7.97e-08}_{-7.68e-08}$ | $0.04^{+0.01}_{NA}$ | 662.3 (1015) | $0.13^{+0.06}_{-0.05}$ | S103 |
| 145 | plaw | $1.44^{+0.57}_{-0.48}$ | 1.13e-06$^{+9.04e-07}_{-4.57e-07}$ | $0.31^{+0.27}_{-0.50}$ | 874.8 (1014) | $1.07^{+0.12}_{-0.12}$ | |
| 146 | plaw | $2.32^{+0.69}_{-0.62}$ | 8.15e-07$^{+7.80e-07}_{-3.78e-07}$ | $0.58^{+0.32}_{-0.27}$ | 724.4 (1014) | $0.25^{+0.09}_{-0.07}$ | S156 |
| 147 | bbod | $0.57^{+0.15}_{-0.12}$ | 2.56e-08$^{+1.51e-08}_{-7.21e-09}$ | $0.74^{+0.69}_{-0.42}$ | 721.5 (1014) | $0.21^{+0.09}_{-0.07}$ | S50 |
| 148 | plaw | $1.93^{+0.33}_{-0.37}$ | 7.92e-07$^{+2.40e-07}_{-1.95e-07}$ | $0.04^{+0.08}_{NA}$ | 744.9 (1014) | $0.55^{+0.12}_{-0.11}$ | VC 149 |
| 149 | bbod | $0.43^{+0.08}_{-0.04}$ | 1.87e-07$^{+2.57e-08}_{-3.93e-08}$ | $0.04^{+0.00}_{NA}$ | 845.8 (1014) | $2.20^{+0.12}_{-0.12}$ | S81; VC 148 |
| 150 | plaw | $1.93^{+1.25}_{-1.12}$ | 3.82e-06$^{+3.69e-05}_{-3.26e-06}$ | $8.07^{+4.08}_{-8.61}$ | 775.7 (1014) | $0.79^{+0.28}_{-0.23}$ | |
| 151 | bbod | $0.34^{+0.06}_{-0.02}$ | 3.12e-07$^{+1.83e-08}_{-6.07e-08}$ | $0.04^{+0.00}_{NA}$ | 961.7 (1014) | $3.43^{+0.12}_{-0.12}$ | S158 |
| 152 | plaw | $1.42^{+0.04}_{-0.04}$ | 4.44e-05$^{+1.95e-06}_{-1.83e-06}$ | $0.12^{+0.01}_{-0.01}$ | 1084.7 (1014) | $47.01^{+0.65}_{-0.65}$ | S146 |
| 153 | plaw | $1.68^{+0.41}_{-0.41}$ | 8.89e-07$^{+4.93e-07}_{-3.15e-07}$ | $0.41^{+0.19}_{-0.18}$ | 824.9 (1014) | $0.61^{+0.14}_{-0.12}$ | S138 |
| 154 | plaw | $2.31^{+0.90}_{-0.66}$ | 9.36e-07$^{+1.77e-06}_{-5.10e-07}$ | $0.95^{+0.68}_{-0.41}$ | 749.0 (1014) | $0.25^{+0.09}_{-0.08}$ | |
| 155 | plaw | $1.70^{f}_{f}$ | 2.87e-07$^{+1.03e-07}_{-8.08e-08}$ | $0.33^{+0.24}_{-0.34}$ | 759.4 (1015) | $0.20^{+0.09}_{-0.07}$ | S75 |
| 156 | plaw | $2.79^{+2.11}_{-1.52}$ | 2.52e-06$^{+4.17e-05}_{-2.12e-06}$ | $1.74^{+2.25}_{-0.69}$ | 780.4 (1014) | $0.31^{+0.13}_{-0.11}$ | |
| 157 | plaw | $2.06^{+0.82}_{-0.66}$ | 3.39e-07$^{+3.14e-07}_{-1.53e-07}$ | $0.18^{+0.22}_{-0.18}$ | 757.3 (1014) | $0.18^{+0.07}_{-0.06}$ | |
| 158 | plaw | $2.69^{+0.68}_{-0.66}$ | 1.54e-06$^{+1.30e-06}_{-6.66e-07}$ | $0.52^{+0.25}_{-0.56}$ | 761.7 (1014) | $0.35^{+0.09}_{-0.08}$ | S91 |
| 159 | plaw | $2.45^{+0.78}_{-0.65}$ | 1.45e-06$^{+1.64e-06}_{-7.03e-07}$ | $0.74^{+0.34}_{-0.29}$ | 894.1 (1014) | $0.36^{+0.10}_{-0.09}$ | |
| 160 | plaw | $1.42^{+0.10}_{-0.11}$ | 7.66e-06$^{+9.00e-07}_{-8.14e-07}$ | $0.20^{+0.04}_{-0.04}$ | 1076.4 (1014) | $7.80^{+0.28}_{-0.28}$ | S141 |
| 161 | plaw | $1.70^{f}_{f}$ | 5.78e-07$^{+2.31e-07}_{-1.70e-07}$ | $1.56^{+0.75}_{NA}$ | 873.0 (1015) | $0.30^{+0.14}_{-0.11}$ | |
| 162 | plaw | $1.65^{+2.27}_{-1.42}$ | 8.97e-07$^{+9.67e-06}_{-7.17e-07}$ | $0.42^{+1.53}_{-0.42}$ | 899.1 (1014) | $0.63^{+0.14}_{-0.13}$ | S119 |
| 163 | plaw | $1.38^{+0.24}_{-0.25}$ | 1.42e-06$^{+4.17e-07}_{-3.24e-07}$ | $0.18^{+0.10}_{-0.09}$ | 925.8 (1014) | $1.54^{+0.13}_{-0.13}$ | S97 |
| 164 | plaw | $2.14^{+1.55}_{-0.96}$ | 3.05e-06$^{+6.94e-06}_{-1.72e-06}$ | $0.17^{+0.42}_{-0.17}$ | 1011.4 (1014) | $1.52^{+0.10}_{-0.10}$ | S159 |
| 165 | plaw | $1.70^{f}_{f}$ | 4.72e-07$^{+2.04e-07}_{-1.54e-07}$ | $1.65^{+0.78}_{-0.62}$ | 757.9 (1015) | $0.24^{+0.13}_{-0.10}$ | |
| 166 | plaw | $2.45^{+0.38}_{-0.37}$ | 6.10e-06$^{+2.54e-06}_{-1.80e-06}$ | $0.34^{+0.14}_{-0.13}$ | 852.0 (1014) | $1.97^{+0.21}_{-0.21}$ | S173; POC 5939–5942 |
| 167 | plaw | $1.63^{+0.26}_{-0.26}$ | 1.79e-06$^{+5.53e-07}_{-4.28e-07}$ | $0.22^{+0.10}_{-0.10}$ | 893.2 (1014) | $1.41^{+0.12}_{-0.12}$ | S124; VC 169 |
| 168 | plaw | $1.50^{+0.14}_{-0.13}$ | 4.88e-06$^{+7.00e-07}_{-5.92e-07}$ | $0.11^{+0.04}_{-0.04}$ | 1020.4 (1014) | $4.73^{+0.20}_{-0.20}$ | S82 |
| 169 | plaw | $1.67^{+0.27}_{-0.26}$ | 1.68e-06$^{+4.99e-07}_{-3.80e-07}$ | $0.18^{+0.09}_{-0.09}$ | 1010.8 (1014) | $1.31^{+0.11}_{-0.11}$ | S121; VC 167 |
| 170 | plaw | $0.19^{+0.68}_{-0.56}$ | 1.86e-07$^{+2.78e-07}_{-1.03e-07}$ | $1.09^{+0.91}_{-0.65}$ | 784.5 (1014) | $1.00^{+0.32}_{-0.27}$ | S74 |
| 171 | plaw | $2.21^{+1.13}_{-0.80}$ | 4.07e-07$^{+6.20e-07}_{-2.16e-07}$ | $0.28^{+0.36}_{-0.26}$ | 769.7 (1014) | $0.17^{+0.08}_{-0.06}$ | |
| 172 | bbod | $0.07^{+0.06}_{-0.01}$ | 9.84e-06$^{+4.48e-01}_{-8.66e-06}$ | $0.69^{+0.49}_{-0.30}$ | 679.6 (1014) | $0.09^{+0.04}_{-0.03}$ | |
| 173 | plaw | $2.06^{+0.91}_{-0.69}$ | 3.26e-07$^{+3.24e-07}_{-1.35e-07}$ | $0.12^{+0.23}_{-0.12}$ | 714.4 (1014) | $0.19^{+0.07}_{-0.06}$ | |

TABLE 6 — *Continued*

| Src Num | Model Type | Γ or kT | Model Normalization | $N_H$ ($10^{22}$ cm$^{-2}$) | C-Stat (DOF) | Luminosity ($10^{37}$ erg s$^{-1}$) | Comments |
|---|---|---|---|---|---|---|---|
| 174 | plaw | $0.82^{+0.24}_{-0.23}$ | $5.16e\text{-}07^{+1.56e-07}_{-1.17e-07}$ | $0.04^{+0.10}_{NA}$ | 863.5 (1014) | $1.22^{+0.14}_{-0.14}$ | S108 |
| 175 | plaw | $1.84^{+0.10}_{-0.09}$ | $4.04e\text{-}05^{+5.43e-06}_{-4.47e-06}$ | $1.06^{+0.08}_{-0.07}$ | 1055.2 (1014) | $18.64^{+0.48}_{-0.48}$ | S57 |
| 176 | plaw | $2.33^{+0.63}_{-0.51}$ | $1.00e\text{-}06^{+6.13e-07}_{-3.49e-07}$ | $0.22^{+0.16}_{-0.37}$ | 815.1 (1014) | $0.40^{+0.10}_{-0.09}$ | S148 |
| 177 | plaw | $1.57^{+0.21}_{-0.21}$ | $2.62e\text{-}06^{+6.86e-07}_{-5.01e-07}$ | $0.22^{+0.08}_{-0.08}$ | 993.7 (1014) | $2.22^{+0.15}_{-0.15}$ | S66 |
| 178 | plaw | $1.51^{+0.09}_{-0.08}$ | $1.87e\text{-}05^{+1.70e-06}_{-1.47e-06}$ | $0.10^{+0.03}_{-0.03}$ | 1117.3 (1014) | $18.28^{+0.41}_{-0.41}$ | S52 |
| 179 | plaw | $1.73^{+0.19}_{-0.19}$ | $9.81e\text{-}06^{+2.48e-06}_{-1.91e-06}$ | $0.58^{+0.11}_{-0.11}$ | 971.5 (1014) | $5.89^{+0.33}_{-0.33}$ | S157; VC 194 |
| 180 | plaw | $1.55^{+0.10}_{-0.09}$ | $9.54e\text{-}06^{+1.01e-06}_{-8.19e-07}$ | $0.10^{+0.03}_{-0.03}$ | 1083.7 (1014) | $8.94^{+0.29}_{-0.29}$ | S145 |
| 181 | plaw | $1.55^{+0.32}_{-0.28}$ | $1.57e\text{-}06^{+5.86e-07}_{-4.02e-07}$ | $0.10^{+0.09}_{-0.08}$ | 969.2 (1014) | $1.47^{+0.13}_{-0.13}$ | S68 |
| 182 | plaw | $2.00^{+0.30}_{-0.26}$ | $4.23e\text{-}06^{+1.51e-06}_{-1.08e-06}$ | $0.51^{+0.14}_{-0.12}$ | 976.3 (1014) | $1.91^{+0.15}_{-0.15}$ | S70 |
| 183 | plaw | $1.17^{+0.03}_{-0.19}$ | $3.96e\text{-}05^{+9.23e-07}_{-6.87e-06}$ | $0.04^{+0.00}_{-0.04}$ | 1201.0 (1014) | $59.14^{+0.88}_{-0.88}$ | S86 |
| 184 | plaw | $1.70^{f}_{f}$ | $1.52e\text{-}07^{+8.73e-08}_{-5.64e-08}$ | $0.25^{+0.35}_{-0.39}$ | 760.9 (1015) | $0.11^{+0.06}_{-0.05}$ | |
| 185 | plaw | $1.70^{f}_{f}$ | $1.77e\text{-}07^{+1.07e-07}_{-7.12e-08}$ | $0.83^{+0.69}_{-0.86}$ | 697.0 (1015) | $0.10^{+0.08}_{-0.05}$ | |
| 186 | plaw | $1.70^{f}_{f}$ | $7.71e\text{-}08^{+4.74e-08}_{-3.24e-08}$ | $0.08^{+0.23}_{NA}$ | 588.2 (1015) | $0.06^{+0.05}_{-0.03}$ | |
| 187 | plaw | $1.70^{f}_{f}$ | $2.95e\text{-}07^{+1.36e-07}_{-9.67e-08}$ | $0.55^{+0.45}_{-0.28}$ | 786.7 (1015) | $0.19^{+0.10}_{-0.08}$ | |
| 188 | plaw | $1.70^{f}_{f}$ | $3.08e\text{-}07^{+1.15e-07}_{-8.71e-08}$ | $0.52^{+0.31}_{-0.22}$ | 806.9 (1015) | $0.20^{+0.10}_{-0.08}$ | |
| 189 | plaw | $1.70^{f}_{f}$ | $3.70e\text{-}07^{+1.55e-07}_{-1.18e-07}$ | $0.16^{+0.23}_{-0.16}$ | 743.8 (1015) | $0.28^{+0.16}_{-0.12}$ | |
| 190 | plaw | $1.65^{+0.65}_{-0.52}$ | $3.56e\text{-}07^{+2.89e-07}_{-1.37e-07}$ | $0.12^{+0.21}_{-0.12}$ | 796.1 (1014) | $0.29^{+0.10}_{-0.08}$ | |
| 191 | bbod | $0.16^{+0.07}_{-0.05}$ | $1.42e\text{-}07^{+2.20e-05}_{-1.10e-07}$ | $1.27^{+1.45}_{-0.69}$ | 768.1 (1014) | $0.04^{+0.03}_{-0.03}$ | |
| 192 | plaw | $1.70^{f}_{f}$ | $3.32e\text{-}07^{+1.44e-07}_{-1.07e-07}$ | $0.41^{+0.31}_{-0.45}$ | 731.6 (1015) | $0.22^{+0.15}_{-0.12}$ | POC 5946–5948 |
| 193 | bbod | $0.15^{+0.03}_{-0.04}$ | $1.88e\text{-}08^{+5.07e-08}_{-7.44e-09}$ | $0.04^{+0.20}_{NA}$ | 695.9 (1014) | $0.11^{+0.05}_{-0.04}$ | S78 |
| 194 | plaw | $1.06^{+0.38}_{-0.55}$ | $4.42e\text{-}07^{+1.31e-07}_{-1.81e-07}$ | $0.04^{+0.02}_{NA}$ | 806.2 (1014) | $0.76^{+0.23}_{-0.20}$ | VC 179 |
| 195 | bbod | $0.20^{+0.05}_{-0.02}$ | $2.49e\text{-}08^{+6.79e-09}_{-8.10e-09}$ | $0.04^{+0.05}_{NA}$ | 789.8 (1014) | $0.20^{+0.06}_{-0.05}$ | |
| 196 | plaw | $1.93^{+1.44}_{-1.02}$ | $1.12e\text{-}06^{+4.10e-06}_{-6.74e-07}$ | $1.24^{+1.22}_{-0.77}$ | 870.3 (1014) | $0.44^{+0.25}_{-0.21}$ | POC 5945, 5946 |
| 197 | plaw | $1.70^{f}_{f}$ | $6.34e\text{-}08^{+3.33e-08}_{-3.22e-08}$ | $0.04^{+0.04}_{NA}$ | 629.4 (1015) | $0.05^{+0.04}_{-0.03}$ | |
| 198 | plaw | $0.86^{+0.93}_{-0.74}$ | $2.77e\text{-}07^{+6.25e-07}_{-1.71e-07}$ | $0.52^{+0.81}_{-0.26}$ | 753.1 (1014) | $0.55^{+0.21}_{-0.17}$ | |
| 199 | bbod | $0.06^{+0.18}_{-0.02}$ | $3.83e\text{-}05^{NA}_{-2.61e-05}$ | $1.08^{+0.61}_{-0.48}$ | 686.0 (1014) | $0.06^{+0.03}_{-0.02}$ | |
| 200 | plaw | $1.70^{f}_{f}$ | $1.46e\text{-}07^{+6.49e-08}_{-4.91e-08}$ | $0.15^{+0.19}_{-0.29}$ | 661.7 (1015) | $0.11^{+0.06}_{-0.05}$ | RS 5937, 5938 |
| 201 | bbod | $0.79^{+0.31}_{-0.23}$ | $1.58e\text{-}08^{+6.57e-09}_{-5.00e-09}$ | $0.15^{+0.79}_{NA}$ | 741.4 (1014) | $0.19^{+0.10}_{-0.08}$ | |
| 202 | plaw | $2.97^{+2.29}_{-0.99}$ | $4.22e\text{-}07^{+8.44e-07}_{-1.83e-07}$ | $0.12^{+0.40}_{-0.12}$ | 748.3 (1014) | $0.14^{+0.06}_{-0.05}$ | |
| 203 | plaw | $2.21^{+0.64}_{-0.52}$ | $1.97e\text{-}06^{+1.20e-06}_{-7.08e-07}$ | $0.20^{+0.17}_{-0.39}$ | 791.9 (1014) | $0.89^{+0.22}_{-0.19}$ | S169 |
| 204 | plaw | $1.62^{+0.46}_{-0.39}$ | $1.00e\text{-}06^{+4.88e-07}_{-2.99e-07}$ | $0.08^{+0.14}_{-0.08}$ | 952.1 (1014) | $0.88^{+0.14}_{-0.14}$ | S137 |
| 205 | plaw | $1.70^{f}_{f}$ | $3.27e\text{-}06^{+5.65e-06}_{-2.78e-06}$ | $48.90^{+30.36}_{-87.37}$ | 704.5 (1015) | $0.28^{+0.21}_{-0.15}$ | RS 5937, 5938 |
| 206 | plaw | $1.81^{+1.27}_{-0.90}$ | $1.18e\text{-}06^{+3.08e-06}_{-7.15e-07}$ | $0.40^{+0.60}_{-0.16}$ | 686.9 (1014) | $0.70^{+0.42}_{-0.34}$ | POC 5945 |
| 207 | bbod | $0.46^{+0.21}_{-0.16}$ | $4.09e\text{-}08^{+6.21e-08}_{-1.22e-08}$ | $0.43^{+0.70}_{-0.37}$ | 767.8 (1014) | $0.34^{+0.14}_{-0.12}$ | S154; POC 5944 |
| 208 | plaw | $1.36^{+0.22}_{-0.28}$ | $1.55e\text{-}06^{+3.70e-07}_{-3.53e-07}$ | $0.04^{+0.08}_{NA}$ | 1001.5 (1014) | $1.87^{+0.21}_{-0.21}$ | S59 |
| 209 | plaw | $1.89^{+0.52}_{-0.43}$ | $2.14e\text{-}06^{+1.21e-06}_{-7.40e-07}$ | $0.17^{+0.18}_{-0.15}$ | 972.2 (1014) | $1.34^{+0.17}_{-0.17}$ | POC 5936 |
| 210 | plaw | $3.93^{+3.37}_{-0.52}$ | $6.09e\text{-}03^{NA}_{-3.72e-03}$ | $44.24^{+35.67}_{-4.65}$ | 1110.6 (1014) | $10.90^{+1.35}_{-1.35}$ | S87 |
| 211 | plaw | $2.55^{+0.74}_{-0.66}$ | $2.59e\text{-}06^{+2.45e-06}_{-1.21e-06}$ | $0.43^{+0.30}_{-0.65}$ | 838.9 (1014) | $0.71^{+0.21}_{-0.18}$ | |
| 212 | bbod | $0.31^{+0.39}_{-0.17}$ | $2.19e\text{-}07^{+2.06e-05}_{-1.25e-07}$ | $1.03^{+1.82}_{-0.51}$ | 750.6 (1014) | $0.72^{+0.33}_{-0.27}$ | S165 |
| 213 | plaw | $0.97^{+1.04}_{-0.82}$ | $1.53e\text{-}06^{+6.07e-06}_{-1.11e-06}$ | $2.35^{+2.22}_{-3.73}$ | 1004.4 (1014) | $2.11^{+0.40}_{-0.40}$ | S73; POC 5949 |
| 214 | plaw | $2.62^{+0.63}_{-0.53}$ | $1.08e\text{-}05^{+7.85e-06}_{-4.14e-06}$ | $0.34^{+0.24}_{-0.51}$ | 794.0 (1014) | $3.05^{+0.77}_{-0.68}$ | S172; POC 5937 |
| 215 | plaw | $1.83^{+1.25}_{-0.92}$ | $2.80e\text{-}06^{+1.31e-05}_{-2.04e-06}$ | $2.19^{+1.84}_{-2.83}$ | 999.2 (1014) | $1.08^{+0.30}_{-0.30}$ | POC 5935 |
| 216 | plaw | $2.17^{+3.89}_{-1.55}$ | $9.61e\text{-}07^{+1.45e-05}_{-7.51e-07}$ | $0.90^{+2.59}_{-0.90}$ | 927.5 (1014) | $0.31^{+0.19}_{-0.16}$ | |
| 217 | plaw | $1.26^{+0.35}_{-0.29}$ | $1.88e\text{-}06^{+8.44e-07}_{-4.32e-07}$ | $0.04^{+0.19}_{NA}$ | 1197.7 (1014) | $2.52^{+0.38}_{-0.38}$ | |
| 218 | plaw | $2.32^{+0.77}_{-0.62}$ | $5.12e\text{-}06^{+5.22e-06}_{-2.29e-06}$ | $0.51^{+0.36}_{-0.62}$ | 1194.3 (1014) | $1.65^{+0.29}_{-0.29}$ | POC 5936, 5949 |
| 219 | plaw | $1.82^{+0.57}_{-0.53}$ | $1.59e\text{-}05^{+1.79e-05}_{-8.11e-06}$ | $1.48^{+0.69}_{-0.55}$ | 1071.9 (1014) | $6.98^{+1.03}_{-1.03}$ | POC 5942 |
| 220 | plaw | $2.31^{+0.58}_{-0.59}$ | $1.49e\text{-}05^{+1.52e-05}_{-7.36e-06}$ | $0.72^{+0.40}_{-0.35}$ | 759.1 (1014) | $4.40^{+1.27}_{-1.08}$ | |
| 221 | plaw | $0.63^{+0.57}_{-0.52}$ | $3.37e\text{-}07^{+3.42e-07}_{-1.48e-07}$ | $0.04^{+0.39}_{NA}$ | 852.1 (1014) | $1.04^{+0.51}_{-0.44}$ | POC 5939–5941 |
| 222 | bbod | $0.09^{+0.04}_{-0.02}$ | $3.06e\text{-}06^{+3.37e-04}_{-2.63e-06}$ | $0.51^{+0.49}_{-0.37}$ | 1003.1 (1014) | $0.53^{+0.19}_{-0.19}$ | |
| 223 | plaw | $2.79^{+3.77}_{-1.39}$ | $6.48e\text{-}06^{+2.28e-04}_{-4.88e-06}$ | $0.85^{+1.79}_{-1.23}$ | 1085.0 (1014) | $1.09^{+0.41}_{-0.41}$ | |
| 224 | bbod | $0.13^{+0.04}_{-0.02}$ | $4.34e\text{-}06^{+2.75e-05}_{-3.47e-06}$ | $0.48^{+0.25}_{-0.29}$ | 653.3 (1014) | $3.13^{+0.74}_{-0.64}$ | S43 |
| 225 | plaw | $1.70^{f}_{f}$ | $2.04e\text{-}07^{+5.56e-08}_{-6.98e-08}$ | $0.04^{+0.05}_{NA}$ | 657.4 (1015) | $0.17^{+0.08}_{-0.06}$ | VC 99 |
| 226 | plaw | $1.77^{+0.32}_{-0.29}$ | $1.26e\text{-}05^{+4.97e-06}_{-3.31e-06}$ | $0.47^{+0.17}_{-0.14}$ | 1083.9 (1014) | $7.54^{+0.64}_{-0.64}$ | POC 5942 |
| 227 | plaw | $1.70^{f}_{f}$ | $9.23e\text{-}08^{+4.23e-08}_{-3.96e-08}$ | $0.04^{+0.15}_{NA}$ | 658.7 (1015) | $0.08^{+0.07}_{-0.05}$ | |
| 228 | plaw | $1.70^{f}_{f}$ | $1.20e\text{-}06^{+6.93e-07}_{-4.92e-07}$ | $0.18^{+0.33}_{NA}$ | 698.5 (1015) | $0.90^{+0.55}_{-0.44}$ | |
| 229 | plaw | $1.70^{f}_{f}$ | $2.94e\text{-}06^{+1.84e-06}_{-1.26e-06}$ | $0.15^{+0.28}_{NA}$ | 398.3 (1015) | $2.25^{+1.66}_{-1.11}$ | S41 |
| 230 | plaw | $1.70^{f}_{f}$ | $1.67e\text{-}06^{+8.40e-07}_{-8.04e-07}$ | $0.04^{+0.06}_{NA}$ | 425.7 (1015) | $1.42^{+1.12}_{-0.73}$ | |
| 231 | plaw | $NA^{NA}_{NA}$ | $0.00e\text{+}00^{+6.06e-05}_{NA}$ | $NA^{NA}_{NA}$ | 1199.0 (1014) | $0.00^{+0.00}_{0.00}$ | S39; POC 5936 |

TABLE 6 — *Continued*

| Src Num | Model Type | Γ or kT | Model Normalization | $N_H$ ($10^{22}$ cm$^{-2}$) | C-Stat (DOF) | Luminosity ($10^{37}$ erg s$^{-1}$) | Comments |
|---|---|---|---|---|---|---|---|
| 232 | bbod | $0.02^{+0.04}_{-0.00}$ | $2.09e-01^{NA}_{NA}$ | $0.09^{+0.86}_{NA}$ | 720.1 (1014) | $1.10^{+1.30}_{-1.10}$ | S36; POC 5935 |
| 233 | bbod | $0.48^{+0.23}_{-0.17}$ | $6.10e-08^{+6.63e-08}_{-2.85e-08}$ | $0.19^{+0.86}_{-0.19}$ | 1245.8 (1014) | $0.63^{+0.37}_{-0.37}$ | S94 |
| 234 | OC | OC | OC | OC | OC | OC | OC |
| 235 | plaw | $1.70^{f}_{f}$ | $1.40e-06^{+6.80e-07}_{-6.25e-07}$ | $0.04^{+0.10}_{NA}$ | 565.2 (1015) | $1.18^{+1.03}_{-0.72}$ | S40; POC 5936 |
| 236 | bbod | $0.10^{+0.07}_{-0.04}$ | $2.01e-07^{+9.11e-04}_{-1.57e-07}$ | $0.25^{+0.85}_{-0.25}$ | 676.0 (1014) | $0.17^{+0.13}_{-0.10}$ | S64; POC 5944 |
| 237 | bbod | $0.65^{+1.01}_{-0.31}$ | $1.05e-07^{+2.31e-05}_{-7.72e-08}$ | $6.98^{+40.06}_{NA}$ | 832.2 (1014) | $0.32^{+1.59}_{-0.32}$ | S76 |
| 238 | plaw | $1.70^{f}_{f}$ | $2.32e-06^{+1.73e-06}_{-1.16e-06}$ | $1.92^{+1.84}_{-2.06}$ | 660.4 (1015) | $1.12^{+3.08}_{-1.12}$ | S47; POC 5937, 5938 |
| 239 | plaw | $1.70^{f}_{f}$ | $1.54e-06^{+9.93e-07}_{-7.25e-07}$ | $0.36^{+0.51}_{-0.65}$ | 591.0 (1015) | $1.04^{+1.21}_{-0.90}$ | S42 |
| 240 | plaw | $1.56^{+0.71}_{-0.45}$ | $9.24e-07^{+1.00e-06}_{-2.99e-07}$ | $0.04^{+0.33}_{NA}$ | 840.5 (1014) | $0.89^{+0.38}_{-0.31}$ | S55; POC 5940, 5941 |
| 241 | OC | OC | OC | OC | OC | OC | OC |
| 242 | plaw | $1.70^{f}_{f}$ | $8.37e-07^{+1.59e-06}_{NA}$ | $0.04^{f}_{0.00}$ | 361.6 (1016) | $0.67^{+2.15}_{-0.67}$ | POC 5935 |
| 243 | bbod | $0.15^{+0.18}_{-0.08}$ | $5.54e-07^{+8.44e-05}_{-4.92e-07}$ | $0.52^{+1.05}_{-0.78}$ | 1007.1 (1014) | $0.60^{+0.65}_{-0.65}$ | S46 |
| 244 | plaw | $2.05^{+2.52}_{-1.29}$ | $1.26e-06^{+3.16e-06}_{-7.02e-07}$ | $0.20^{+0.42}_{-0.20}$ | 1080.8 (1014) | $0.66^{+0.36}_{-0.36}$ | S77 |
| 245 | plaw | $1.70^{f}_{f}$ | $8.96e-05^{+3.17e-04}_{-7.56e-05}$ | $65.45^{+62.70}_{-37.22}$ | 453.2 (1015) | $5.26^{+21.29}_{-5.26}$ | S38 |
| 246 | plaw | $1.70^{f}_{f}$ | $1.52e-07^{+1.54e-07}_{-9.57e-08}$ | $0.04^{f}_{0.00}$ | 666.8 (1016) | $0.12^{+0.88}_{-0.12}$ | S45; POC 5937, 5938 |
| 247 | plaw | $NA^{NA}_{NA}$ | $0.00e+00^{+1.73e-08}_{NA}$ | $NA^{f}_{NA}$ | 566.7 (1016) | $0.00^{+0.00}_{0.00}$ | |
| 248 | plaw | $1.70^{f}_{f}$ | $1.24e-08^{+1.89e-08}_{NA}$ | $0.04^{f}_{0.00}$ | 596.0 (1016) | $0.01^{+0.21}_{-0.01}$ | S123 |
| 249 | plaw | $1.70^{f}_{f}$ | $4.18e-19^{+1.33e-08}_{NA}$ | $0.04^{f}_{0.00}$ | 621.3 (1016) | $0.00^{+0.00}_{0.00}$ | S133 |
| 250 | plaw | $1.70^{f}_{f}$ | $4.76e-08^{+5.37e-08}_{-3.14e-08}$ | $0.41^{+0.76}_{NA}$ | 602.7 (1015) | $0.03^{+0.09}_{-0.03}$ | S114 |
| 251 | plaw | $1.70^{f}_{f}$ | $7.76e-07^{+5.07e-07}_{-3.22e-07}$ | $8.74^{+4.78}_{-3.38}$ | 642.7 (1015) | $0.23^{+0.20}_{-0.13}$ | RS 5943 |
| 252 | plaw | $1.70^{f}_{f}$ | $1.11e-07^{+6.24e-08}_{-4.54e-08}$ | $0.08^{+0.21}_{NA}$ | 614.7 (1015) | $0.09^{+0.07}_{-0.05}$ | S107 |
| 253 | plaw | $1.70^{f}_{f}$ | $5.35e-06^{+4.99e-03}_{NA}$ | $162.90^{NA}_{-162.90}$ | 635.6 (1015) | $0.05^{+0.00}_{0.00}$ | S95 |
| 254 | plaw | $1.70^{f}_{f}$ | $6.81e-08^{+1.32e-07}_{-6.12e-08}$ | $2.44^{+5.21}_{-3.84}$ | 669.9 (1015) | $0.03^{+0.00}_{0.00}$ | S92 |
| 255 | plaw | $NA^{NA}_{NA}$ | $0.00e+00^{+9.97e-09}_{NA}$ | $NA^{f}_{NA}$ | 624.5 (1016) | $0.00^{+0.00}_{0.00}$ | S89 |
| 256 | bbod | $0.26^{+0.16}_{-0.16}$ | $5.41e-09^{+1.24e-07}_{-2.37e-09}$ | $0.04^{+2.42}_{NA}$ | 821.2 (1014) | $0.05^{+0.04}_{-0.03}$ | S153 |
| 257 | plaw | $1.70^{f}_{f}$ | $4.19e-08^{+2.72e-08}_{-2.35e-08}$ | $0.04^{+0.05}_{NA}$ | 672.2 (1015) | $0.04^{+0.04}_{-0.03}$ | |
| 258 | plaw | $1.70^{f}_{f}$ | $1.46e-07^{+4.41e-06}_{NA}$ | $9.16^{NA}_{-9.16}$ | 733.6 (1015) | $0.04^{+0.41}_{-0.04}$ | S174 |
| 259 | plaw | $1.70^{f}_{f}$ | $8.65e-08^{+3.80e-08}_{-3.98e-08}$ | $0.04^{+0.03}_{NA}$ | 663.9 (1015) | $0.07^{+0.05}_{-0.04}$ | |
| 260 | plaw | $1.70^{f}_{f}$ | $5.65e-07^{+4.78e-07}_{-2.79e-07}$ | $8.62^{+6.14}_{-3.89}$ | 651.4 (1015) | $0.17^{+0.19}_{-0.13}$ | RS 5945 |
| 261 | bbod | $0.09^{+0.08}_{-0.03}$ | $8.11e-07^{+1.86e-03}_{-7.65e-07}$ | $1.03^{+1.16}_{-0.82}$ | 636.5 (1014) | $0.02^{+0.02}_{-0.02}$ | S149; RS 5949 |
| 262 | OC | OC | OC | OC | OC | OC | OC |
| 263 | plaw | $NA^{NA}_{NA}$ | $0.00e+00^{+2.05e-01}_{NA}$ | $NA^{NA}_{NA}$ | 663.1 (1015) | $0.00^{+0.00}_{0.00}$ | S129 |
| 264 | plaw | $1.44^{+0.10}_{-0.09}$ | $8.98e-06^{+9.56e-07}_{-8.16e-07}$ | $0.12^{+0.04}_{-0.03}$ | 933.3 (1014) | $9.32^{+0.31}_{-0.31}$ | |
| 265 | plaw | $2.06^{+1.78}_{-1.08}$ | $4.91e-07^{+1.09e-06}_{-3.03e-07}$ | $0.32^{+0.45}_{-0.32}$ | 765.6 (1014) | $0.23^{+0.13}_{-0.10}$ | |
| B1 | bbod | $0.83^{+0.93}_{-0.34}$ | $6.82e-07^{+3.39e-06}_{-3.17e-07}$ | $7.29^{+9.30}_{-4.45}$ | 1152.2 (1014) | $3.11^{+1.48}_{-1.48}$ | |
| B2 | plaw | $1.70^{f}_{f}$ | $1.11e-07^{NA}_{NA}$ | $0.43^{NA}_{-0.43}$ | 746.8 (1015) | $0.07^{+0.08}_{-0.06}$ | |
| B3 | plaw | $1.70^{f}_{f}$ | $4.35e-07^{+2.21e-07}_{-1.64e-07}$ | $2.25^{+1.27}_{-1.01}$ | 680.2 (1015) | $0.20^{+0.13}_{-0.09}$ | |
| B4 | plaw | $1.70^{f}_{f}$ | $1.16e-07^{+6.60e-08}_{-4.59e-08}$ | $0.15^{+0.24}_{NA}$ | 633.5 (1015) | $0.09^{+0.06}_{-0.04}$ | |
| B5 | plaw | $1.70^{f}_{f}$ | $8.51e-08^{NA}_{NA}$ | $0.04^{NA}_{NA}$ | 890.5 (1015) | $0.07^{+0.05}_{-0.04}$ | |
| B6 | plaw | $1.70^{f}_{f}$ | $6.85e-08^{+4.16e-08}_{-3.76e-08}$ | $0.04^{+0.14}_{NA}$ | 670.6 (1015) | $0.06^{+0.06}_{-0.04}$ | |
| B7 | plaw | $1.70^{f}_{f}$ | $6.61e-07^{+4.67e-07}_{-2.77e-07}$ | $2.12^{+3.63}_{-0.91}$ | 797.7 (1015) | $0.31^{+0.25}_{-0.21}$ | POC 5935 |
| B8 | OC | OC | OC | OC | OC | OC | OC |
| B9 | OC | OC | OC | OC | OC | OC | OC |
| B10 | plaw | $1.70^{f}_{f}$ | $1.62e-07^{+1.65e-07}_{-8.91e-08}$ | $1.73^{+1.83}_{-2.14}$ | 690.7 (1015) | $0.08^{+0.12}_{-0.08}$ | |
| B11 | bbod | $0.19^{+0.12}_{-0.07}$ | $1.21e-03^{NA}_{-1.21e-03}$ | $28.12^{+25.92}_{-40.77}$ | 745.0 (1014) | $0.10^{+0.08}_{-0.07}$ | |

NOTE. — Column 1: Source number. A "B" before the number refers to a borderline source not part of the master source list. Column 2: The model used for fitting the spectrum ("plaw" = power law and "bbod" = blackbody). Column 3: Γ = Powerlaw Index, kT = Blackbody Temperature (keV) of the best-fit model. Column 4: "Model Normalization" is the model normalization in units of photons keV$^{-1}$ cm$^{-2}$ s$^{-1}$ at 1 keV for the power-law model and $L_{39}/(D_{10})^2$, where $L_{39}$ is the source luminosity in units of $10^{39}$ erg s$^{-1}$ and $D_{10}$ is the distance to the source in units of 10 kpc for the blackbody model. Column 5: The best-fit column density for the source which includes galactic foreground and intrinsic source absorption. A value is "0.04" indicates that the best-fit is on the galactic foreground minimum column density (the lower bound will then be "NA"). Column 6: "C-stat (DOF)" is the total best-fit C-statistic and number of degrees of freedom for the source and background models together. Column 7: The 0.5–8.0 keV luminosity calculated from the best fit model. The uncertainties are estimated by scaling the luminosity by the uncertainty in the counts, which was calculated from the 90% Bayesian confidence intervals, (Kraft et al. 1991). Column 8: Other details about the source extraction.
Abbreviations of table values: "OC" = "Off Chip". "NA" = "Not Applicable/Available". This occurs when: in the case of source 62, the model is too complicated to be listed in the table; Sherpa fails to find the confidence interval; the source has zero flux so that Γ or kT is not defined. An "f" indicates that the parameter was frozen during the spectral fitting. "RS ObsID" indicates that the source was on the readout streak in the specified ObsID. "POC ObsID" indicates that the source was partially off of the chip in the specified ObsID. "S#" indicates the Swartz source number that this source is matched to. "VC #" indicates that the source was very close to another source.
(†) Sherpa's JD pileup model (Davis 2001) was used in addition to the power-law fit
(‡) See Swartz et al. (2003) for model parameters
